# Supplementary material for: Breaking Down the Lockdown: The Causal Effects of Stay-At-Home Mandates on Uncertainty and Sentiments During the COVID-19 Pandemic
Source: arXiv:2212.01705 source file (2023-06-01)
Supplement: Supplementary file 1 [file additional_material.tex]

\documentclass[../main.tex]{subfiles}
\begin{document}

We show the results including December 2019 in the pre-treatment period.

\begin{table}[H]\centering
\def\sym#1{\ifmmode^{#1}\else\(^{#1}\)\fi}
\caption{Regression estimates of model (1) for \emph{Uncertainty} and \emph{Negative Sentiment}, aggregated and grouped by topics. \label{did_1}}
\begin{adjustbox}{max width=\textwidth}
\begin{tabular}{lrrrrrrrrrr}
\toprule
&\multicolumn{5}{c}{Uncertainty}&\multicolumn{5}{c}{Negative Sentiment}\\
\toprule
                    &\multicolumn{1}{c}{(1)}&\multicolumn{1}{c}{(2)}&\multicolumn{1}{c}{(3)}&\multicolumn{1}{c}{(4)}&\multicolumn{1}{c}{(5)}&\multicolumn{1}{c}{(6)}&\multicolumn{1}{c}{(7)}&\multicolumn{1}{c}{(8)}&\multicolumn{1}{c}{(9)}&\multicolumn{1}{c}{(10)}\\
                    &\multicolumn{1}{c}{Aggregate}&\multicolumn{1}{c}{Economics}&\multicolumn{1}{c}{Health}&\multicolumn{1}{c}{Politics}&\multicolumn{1}{c}{Lockdown Pol.}&\multicolumn{1}{c}{Aggregate}&\multicolumn{1}{c}{Economics}&\multicolumn{1}{c}{Health}&\multicolumn{1}{c}{Politics}&\multicolumn{1}{c}{Lockdown Pol.}\\
\midrule
zonarossa=1         &      0.0606         &      0.0139\sym{*}  &     0.00652         &     -0.0140\sym{**} &     0.00167         &       0.108         &      0.0169\sym{*}  &     0.00193         &     -0.0420\sym{***}&    0.000269         \\
                    &      (0.81)         &      (2.20)         &      (0.93)         &     (-3.28)         &      (0.37)         &      (1.95)         &      (2.31)         &      (0.40)         &     (-4.34)         &      (0.19)         \\
\addlinespace
post=1              &      0.0545\sym{**} &     0.00705\sym{**} &      0.0610\sym{***}&    -0.00259         &      0.0195\sym{***}&     -0.0501         &    -0.00726\sym{***}&      0.0317\sym{***}&     -0.0146         &     0.00460\sym{*}  \\
                    &      (3.31)         &      (2.75)         &      (5.50)         &     (-0.49)         &      (8.55)         &     (-1.03)         &     (-3.50)         &      (4.84)         &     (-1.46)         &      (2.56)         \\
\addlinespace
post=2              &      0.0673\sym{***}&      0.0139\sym{***}&      0.0695\sym{***}&    -0.00284         &      0.0188\sym{***}&     -0.0661         &   -0.000719         &      0.0381\sym{***}&     -0.0229\sym{*}  &     0.00673\sym{*}  \\
                    &      (4.18)         &      (4.37)         &      (7.07)         &     (-0.56)         &      (5.78)         &     (-1.55)         &     (-0.25)         &      (6.66)         &     (-2.60)         &      (2.36)         \\
\addlinespace
zonarossa=1 $\times$ post=1&      0.0231         &     -0.0149         &      0.0320\sym{*}  &      0.0153\sym{*}  &     0.00300         &     0.00789         &     -0.0109         &      0.0521\sym{***}&      0.0507\sym{***}&      0.0124         \\
                    &      (0.22)         &     (-1.75)         &      (2.27)         &      (2.19)         &      (0.22)         &      (0.16)         &     (-1.16)         &      (4.18)         &      (4.21)         &      (1.17)         \\
\addlinespace
zonarossa=1 $\times$ post=2&     -0.0248         &     -0.0132         &     -0.0142         &     0.00612         &    -0.00883\sym{*}  &      0.0510         &     0.00131         &      0.0424         &      0.0717\sym{***}&     0.00777         \\
                    &     (-0.39)         &     (-1.61)         &     (-0.67)         &      (1.00)         &     (-2.08)         &      (0.90)         &      (0.08)         &      (1.79)         &      (4.46)         &      (1.35)         \\
\addlinespace
Constant            &       0.195\sym{***}&      0.0145\sym{***}&     0.00768\sym{***}&      0.0197\sym{***}&     0.00402\sym{***}&       0.347\sym{***}&      0.0229\sym{***}&     0.00943\sym{***}&      0.0449\sym{***}&     0.00541\sym{***}\\
                    &     (14.69)         &      (8.66)         &     (10.00)         &      (4.64)         &      (5.07)         &      (8.41)         &      (8.92)         &      (9.21)         &      (4.75)         &      (4.32)         \\
\midrule
Observations        &       29819         &       29819         &       29819         &       29819         &       29819         &       29819         &       29819         &       29819         &       29819         &       29819         \\
\midrule
Clustered SE & Yes & Yes & Yes & Yes & Yes & Yes & Yes & Yes & Yes & Yes \\ 
\bottomrule
\multicolumn{11}{l}{\footnotesize \textit{t} statistics in parentheses}\\
\multicolumn{11}{l}{\footnotesize \sym{*} \(p<0.05\), \sym{**} \(p<0.01\), \sym{***} \(p<0.001\)}\\
\end{tabular}
\end{adjustbox}
\end{table}

\begin{table}[H]\centering
\def\sym#1{\ifmmode^{#1}\else\(^{#1}\)\fi}
\caption{Benjamini Hochberg (1995) adjusted p-values (original p-values in parenthesis)\label{adj_p1}}
\begin{adjustbox}{max width=\textwidth}
\begin{tabular}{lrrrrrrrrrr}
\toprule 
\multicolumn{1}{c}{}&\multicolumn{5}{c}{\textbf{Uncertainty}}&\multicolumn{5}{c}{\textbf{Negative Sentiment}}\\
\toprule
         &\multicolumn{1}{c}{Aggregate}&\multicolumn{1}{c}{Economics}&\multicolumn{1}{c}{Health}&\multicolumn{1}{c}{Politics}&\multicolumn{1}{c}{Lockdown Pol}&\multicolumn{1}{c}{Aggregate}&\multicolumn{1}{c}{Economics}&\multicolumn{1}{c}{Health}&\multicolumn{1}{c}{Politics}&\multicolumn{1}{c}{Lockdown Pol}\\
\midrule
red zone = 1 & 0.52 & 0.06 & 0.47 & 0.00 & 0.75 & 0.13 & 0.04 & 0.81 & 0.00 & 0.89 \\
            & (0.42) & (0.03) & (0.35)& (0.00) & (0.71) & (0.05) & (0.02) & (0.69)& (0.00) & (0.85)\\
post = 1     & 0.00 & 0.02 & 0.00  & 0.69  &  0.00 & 0.51 & 0.00 & 0.00 & 0.22 & 0.02\\
           & (0.00) & (0.01) & (0.00)& (0.63) & (0.00) & (0.30) & (0.00) & (0.00)& (0.14) & (0.01)\\
post = 2   & 0.00 & 0.00& 0.00 & 0.68 & 0.00 & 0.26 & 0.89 & 0.00  & 0.02 & 0.04\\
            & (0.00) & (0.00) & (0.00)& (0.57) & (0.00) & (0.12) & (0.81) & (0.00)& (0.01) & (0.02)\\
\textbf{red zone = 1 x post = 1}  & 0.82 & 0.13 & 0.06 & 0.06 & 0.83 & 0.87 & 0.31 & 0.00 & 0.00 & 0.31 \\
& (0.82) & (0.08) & (0.02)& (0.03) & (0.83) & (0.87) & (0.25) & (0.00)& (0.00) & (0.24)\\
red zone = 1 x post = 2 & 0.75 & 0.17 & 0.63 & 0.45 & 0.07 & 0.53 & 0.94 & 0.12  & 0.00 & 0.25 \\
            & (0.70) & (0.11) & (0.50)& (0.32) & (0.04) & (0.37) & (0.94) & (0.07)& (0.00) & (0.18)\\
\bottomrule
\end{tabular}
\end{adjustbox}
\end{table}

\begin{table}[H]\centering
\def\sym#1{\ifmmode^{#1}\else\(^{#1}\)\fi}
\caption{Estimates of spillover effect and total treat effect for \emph{Uncertainty} and \emph{Negative Sentiment} in model (12) , with clustered standard errors.}
\begin{adjustbox}{max width=\textwidth}
\begin{tabular}{lrrrrrrrrrr}
\toprule
&\multicolumn{5}{c}{Uncertainty}&\multicolumn{5}{c}{Negative Sentiment}\\
\toprule
                    &\multicolumn{1}{c}{(1)}&\multicolumn{1}{c}{(2)}&\multicolumn{1}{c}{(3)}&\multicolumn{1}{c}{(4)}&\multicolumn{1}{c}{(5)}&\multicolumn{1}{c}{(6)}&\multicolumn{1}{c}{(7)}&\multicolumn{1}{c}{(8)}&\multicolumn{1}{c}{(9)}&\multicolumn{1}{c}{(10)}\\
                    &\multicolumn{1}{c}{Aggregate}&\multicolumn{1}{c}{Economics}&\multicolumn{1}{c}{Health}&\multicolumn{1}{c}{Politics}&\multicolumn{1}{c}{Lockdown Pol.}&\multicolumn{1}{c}{Aggregate}&\multicolumn{1}{c}{Economics}&\multicolumn{1}{c}{Health}&\multicolumn{1}{c}{Politics}&\multicolumn{1}{c}{Lockdown Pol.}\\
\midrule
zonarossa=1         &      0.0629         &      0.0124         &     0.00161         &     -0.0115\sym{*}  &    -0.00173         &       0.118\sym{*}  &      0.0156         &     -0.0101         &     -0.0392\sym{***}&    -0.00693         \\
                    &      (0.84)         &      (1.62)         &      (0.14)         &     (-2.21)         &     (-0.32)         &      (2.13)         &      (1.93)         &     (-1.27)         &     (-3.98)         &     (-1.72)         \\
\addlinespace
post=1              &      0.0592\sym{***}&     0.00844\sym{***}&      0.0658\sym{***}&   -0.000996         &      0.0205\sym{***}&     -0.0488         &    -0.00613\sym{***}&      0.0321\sym{***}&     -0.0126         &     0.00507\sym{**} \\
                    &      (4.79)         &      (4.85)         &      (7.72)         &     (-0.24)         &     (12.72)         &     (-1.12)         &     (-3.52)         &      (5.28)         &     (-1.46)         &      (2.87)         \\
\addlinespace
post=2              &      0.0713\sym{***}&      0.0152\sym{***}&      0.0739\sym{***}&    -0.00122         &      0.0198\sym{***}&     -0.0654         &    0.000275         &      0.0382\sym{***}&     -0.0209\sym{**} &     0.00699\sym{*}  \\
                    &      (5.48)         &      (5.64)         &      (9.62)         &     (-0.32)         &      (7.56)         &     (-1.67)         &      (0.09)         &      (6.87)         &     (-2.74)         &      (2.56)         \\
\addlinespace
zonarossa=1 $\times$ post=1&      0.0185         &     -0.0163         &      0.0271\sym{*}  &      0.0137\sym{*}  &     0.00198         &     0.00658         &     -0.0120         &      0.0517\sym{***}&      0.0488\sym{***}&      0.0120         \\
                    &      (0.18)         &     (-1.96)         &      (2.22)         &      (2.21)         &      (0.14)         &      (0.15)         &     (-1.28)         &      (4.23)         &      (4.44)         &      (1.12)         \\
\addlinespace
zonarossa=1 $\times$ post=2&     -0.0288         &     -0.0145         &     -0.0186         &     0.00451         &    -0.00975\sym{*}  &      0.0503         &    0.000311         &      0.0423         &      0.0697\sym{***}&     0.00750         \\
                    &     (-0.46)         &     (-1.80)         &     (-0.91)         &      (0.87)         &     (-2.59)         &      (0.93)         &      (0.02)         &      (1.79)         &      (4.51)         &      (1.32)         \\
\addlinespace
$\eta_{(0,20]}$&     -0.0177         &    -0.00191         &    -0.00899         &     0.00463         &    -0.00162         &     -0.0300         &    -0.00271         &    -0.00957         &     0.00560         &    -0.00650         \\
                    &     (-0.63)         &     (-0.40)         &     (-1.35)         &      (1.07)         &     (-0.53)         &     (-0.51)         &     (-0.62)         &     (-0.99)         &      (0.62)         &     (-1.55)         \\
\addlinespace
$\eta_{(20,25]}$&    -0.00845         &     -0.0104\sym{*}  &     -0.0334\sym{***}&     -0.0101\sym{**} &     -0.0122\sym{***}&      0.0421         &    -0.00734         &     -0.0175\sym{**} &     -0.0131         &     -0.0113\sym{**} \\
                    &     (-0.68)         &     (-2.15)         &     (-4.49)         &     (-2.62)         &     (-3.98)         &      (1.56)         &     (-1.78)         &     (-2.72)         &     (-1.93)         &     (-2.89)         \\
\addlinespace
$\eta_{(25,30]}$&      0.0249         &     0.00251         &      0.0104         &     0.00668         &    -0.00168         &      0.0325         &     0.00245         &     -0.0136\sym{*}  &     0.00771         &    -0.00717         \\
                    &      (1.71)         &      (0.53)         &      (1.32)         &      (1.43)         &     (-0.48)         &      (0.72)         &      (0.42)         &     (-2.25)         &      (0.67)         &     (-1.86)         \\
\addlinespace
Constant            &       0.193\sym{***}&      0.0160\sym{***}&      0.0126         &      0.0172\sym{**} &     0.00741\sym{*}  &       0.337\sym{***}&      0.0241\sym{***}&      0.0214\sym{***}&      0.0421\sym{***}&      0.0126\sym{**} \\
                    &     (12.42)         &      (3.44)         &      (1.45)         &      (3.33)         &      (2.28)         &      (8.24)         &      (5.62)         &      (3.39)         &      (4.37)         &      (3.17)         \\
\midrule
Observations        &       29819         &       29819         &       29819         &       29819         &       29819         &       29819         &       29819         &       29819         &       29819         &       29819         \\
\bottomrule
\multicolumn{11}{l}{\footnotesize \textit{t} statistics in parentheses}\\
\multicolumn{11}{l}{\footnotesize \sym{*} \(p<0.05\), \sym{**} \(p<0.01\), \sym{***} \(p<0.001\)}\\
\end{tabular}
\end{adjustbox}
\end{table}

Again we look for indirect evidence supporting the parallel trends assumption between treated and controls and estimate again model (13) including December 2019 in the analysis in \ref{pt_1}.
We take the period going from Feb. 1st to Feb. 19th 2020 as baseline (post=0) and define time dummies for December 2019 (post=1), January 2020 (post=2), Feb. 23rd -  March 6th (post=3) - the first post-treatment period, and from March 9th to March 16th (post=4). 

%We consider five pre-treatment periods and 3 post-treatment period. 

%In Figures \ref{fig:pt_1} and \ref{fig:pt_2}, we report the coefficient estimates of $\gamma_{j}$ along with 95 percent confidence intervals. The models for aggregated uncertainty and negative sentiments seem to fail the parallel-trend assumption, as the coefficient estimates are significantly different from zero, in particular around three or two days before the lockdown. Considering uncertainty and negative sentiment grouped by topics, there is a common anticipatory effects of the treated units around one day before the lockdown. This should come as unexpected, as the government announced the restriction policy a day before the beginning of the lockdown.

%In Figures \ref{fig:pt_4} and \ref{fig:pt_5}, we report the adjusted Benjamini-Hochberg p-values \cite{BH}, obtained by jointly testing independent regressions as described in Section 6.1, along with unadjusted p-values, of the $\gamma_{j}$ coefficient estimates. The corrected p-values do not substantially alter the previous results, except for uncertainty, as the coefficients loose significance as we go beyond three days before the lockdown. 

\begin{figure}[H]
  \begin{subfigure}[h]{0.4\textwidth}
    \includegraphics[width=\textwidth]{figures/parallel_trends_wt_december/pt_unc.png}
    \caption{Uncertainty}
    \label{fig:pt_1asm}
  \end{subfigure}
  \hfill
 \begin{subfigure}[h]{0.4\textwidth}
    \includegraphics[width=\textwidth]{figures/parallel_trends_wt_december/pt_sent.png}
    \caption{Negative Sentiment}
    \label{fig:pt_1bsm}
  \end{subfigure}
  \caption{Coefficient Estimates and Confidence Intervals (\% 95) of interaction between the treatment variable and time dummies. The dependent variable is Share of tweets classified as \emph{Uncertainty} (a) and \emph{Negative sentiment} (b). The baseline period starts from the 1rst of February and ends on the 19th of February.}
  \label{fig:pt_1sm}
\end{figure}

\begin{figure}[H]
  \begin{subfigure}[h]{0.4\textwidth}
    \includegraphics[width=\textwidth]{figures/parallel_trends_wt_december/pt_unc_e.png}
    \caption{Uncertainty-Economics}
    \label{fig:pt_2asm}
  \end{subfigure}
  \hfill
 \begin{subfigure}[h]{0.4\textwidth}
    \includegraphics[width=\textwidth]{figures/parallel_trends_wt_december/pt_unc_h.png}
    \caption{Uncertainty-Health}
    \label{fig:pt_2bsm}
  \end{subfigure}
  \begin{subfigure}[h]{0.4\textwidth}
    \includegraphics[width=\textwidth]{figures/parallel_trends_wt_december/pt_unc_p.png}
    \caption{Uncertainty-Politics}
    \label{fig:pt_2csm}
  \end{subfigure}
  \hfill
 \begin{subfigure}[h]{0.4\textwidth}
    \includegraphics[width=\textwidth]{figures/parallel_trends_wt_december/pt_unc_l.png}
    \caption{Uncertainty-Lockdown restrictions}
    \label{fig:pt_2dsm}
  \end{subfigure}
    \begin{subfigure}[h]{0.4\textwidth}
    \includegraphics[width=\textwidth]{figures/parallel_trends_wt_december/pt_ns_e.png}
    \caption{Negative Sentiment-Economics}
    \label{fig:pt_3asm}
  \end{subfigure}
  \hfill
 \begin{subfigure}[h]{0.4\textwidth}
    \includegraphics[width=\textwidth]{figures/parallel_trends_wt_december/pt_ns_h.png}
    \caption{Negative Sentiment-Health}
    \label{fig:pt_3bsm}
  \end{subfigure}
  \begin{subfigure}[h]{0.4\textwidth}
    \includegraphics[width=\textwidth]{figures/parallel_trends_wt_december/pt_ns_p.png}
    \caption{Negative Sentiment-Politics}
    \label{fig:pt_3csm}
  \end{subfigure}
  \hfill
 \begin{subfigure}[h]{0.4\textwidth}
    \includegraphics[width=\textwidth]{figures/parallel_trends_wt_december/pt_ns_l.png}
    \caption{Negative Sentiment-Lockdown restrictions}
    \label{fig:pt_3dsm}
  \end{subfigure}
  \caption{Coefficient Estimates and Confidence Intervals (\% 95) of interaction between the treatment variable and time dummies. The dependent variable is Share of tweets classified as \emph{Uncertainty} and \emph{Negative Sentiment} grouped by Topic. The baseline period starts from the 1rst of February and ends on the 19th of February.}
  \label{fig:pt_2sm}
\end{figure}

\begin{table}[H]\centering
\def\sym#1{\ifmmode^{#1}\else\(^{#1}\)\fi}
\caption{DID model with leads and lags of the treatment for \emph{Uncertainty} and \emph{Negative Sentiment}, aggregated and grouped by topics.\label{pt_1}}
\begin{adjustbox}{max width=\textwidth}
\begin{tabular}{lrrrrrrrrrr}
\toprule
&\multicolumn{5}{c}{Uncertainty}&\multicolumn{5}{c}{Negative Sentiment}\\
\toprule
                    &\multicolumn{1}{c}{(1)}&\multicolumn{1}{c}{(2)}&\multicolumn{1}{c}{(3)}&\multicolumn{1}{c}{(4)}&\multicolumn{1}{c}{(5)}&\multicolumn{1}{c}{(6)}&\multicolumn{1}{c}{(7)}&\multicolumn{1}{c}{(8)}&\multicolumn{1}{c}{(9)}&\multicolumn{1}{c}{(10)}\\
                    &\multicolumn{1}{c}{Aggregate}&\multicolumn{1}{c}{Economics}&\multicolumn{1}{c}{Health}&\multicolumn{1}{c}{Politics}&\multicolumn{1}{c}{Lockdown Pol.}&\multicolumn{1}{c}{Aggregate}&\multicolumn{1}{c}{Economics}&\multicolumn{1}{c}{Health}&\multicolumn{1}{c}{Politics}&\multicolumn{1}{c}{Lockdown Pol.}\\
\midrule
\addlinespace
post=1              &    -0.00969         &     0.00176         &    -0.00559\sym{*}  &  0.00000752         &     0.00192         &      0.0270         &    0.000676         &     0.00242         &     0.00210         &     0.00384         \\
                    &     (-0.54)         &      (0.93)         &     (-2.50)         &      (0.00)         &      (0.99)         &      (0.56)         &      (0.25)         &      (0.82)         &      (0.30)         &      (1.96)         \\
\addlinespace
post=2              &      0.0206         &    0.000267         &    -0.00149         &     0.00698         &    0.000948         &       0.108         &     0.00964         &     0.00623         &      0.0150         &     0.00347\sym{**} \\
                    &      (0.88)         &      (0.08)         &     (-0.90)         &      (0.63)         &      (0.61)         &      (1.84)         &      (1.07)         &      (1.85)         &      (1.13)         &      (2.80)         \\
\addlinespace
post=3              &      0.0573\sym{***}&     0.00753\sym{**} &      0.0593\sym{***}&   -0.000883         &      0.0201\sym{***}&     -0.0174         &    -0.00474         &      0.0338\sym{***}&     -0.0104         &     0.00634\sym{**} \\
                    &      (5.46)         &      (3.10)         &      (5.56)         &     (-0.46)         &      (9.10)         &     (-0.55)         &     (-1.28)         &      (5.23)         &     (-1.69)         &      (3.19)         \\
\addlinespace
post=4              &      0.0701\sym{***}&      0.0144\sym{***}&      0.0678\sym{***}&    -0.00113         &      0.0195\sym{***}&     -0.0334         &     0.00179         &      0.0402\sym{***}&     -0.0188\sym{**} &     0.00847\sym{**} \\
                    &      (5.56)         &      (4.45)         &      (7.20)         &     (-0.46)         &      (6.05)         &     (-1.06)         &      (0.47)         &      (6.88)         &     (-3.32)         &      (2.76)         \\
\addlinespace
zonarossa=1         &     -0.0478\sym{**} &     -0.0140\sym{***}&    -0.00935\sym{***}&    -0.00691         &    -0.00334\sym{***}&       0.119         &     0.00186         &    -0.00734\sym{***}&     -0.0407\sym{***}&    -0.00367\sym{**} \\
                    &     (-3.15)         &     (-6.61)         &     (-6.43)         &     (-1.19)         &     (-4.73)         &      (1.54)         &      (0.18)         &     (-7.04)         &     (-5.71)         &     (-2.66)         \\
\addlinespace
post=1 $\times$ zonarossa=1&       0.128         &      0.0321         &      0.0310\sym{***}&    -0.00264         &     0.00655         &     -0.0620         &     0.00253         &      0.0145\sym{**} &     0.00637         &     0.00463         \\
                    &      (1.26)         &      (1.86)         &     (12.71)         &     (-0.26)         &      (1.39)         &     (-0.85)         &      (0.25)         &      (3.18)         &      (0.78)         &      (0.58)         \\
\addlinespace
post=2 $\times$ zonarossa=1&       0.154         &      0.0414\sym{***}&      0.0154         &     -0.0181         &     0.00600         &     -0.0275         &      0.0306\sym{**} &     0.00766         &     -0.0150         &     0.00347         \\
                    &      (1.84)         &      (5.31)         &      (1.39)         &     (-1.51)         &      (1.06)         &     (-0.39)         &      (3.15)         &      (0.67)         &     (-1.13)         &      (0.62)         \\
\addlinespace
post=3 $\times$ zonarossa=1&       0.132\sym{***}&      0.0130\sym{***}&      0.0478\sym{***}&     0.00817         &     0.00801         &    -0.00359         &     0.00416         &      0.0614\sym{***}&      0.0494\sym{***}&      0.0164         \\
                    &      (4.44)         &      (3.88)         &      (3.82)         &      (1.10)         &      (0.83)         &     (-0.09)         &      (0.34)         &      (6.80)         &      (5.70)         &      (1.61)         \\
\addlinespace
post=4 $\times$ zonarossa=1&      0.0837\sym{***}&      0.0147\sym{*}  &     0.00166         &    -0.00101         &    -0.00383         &      0.0395         &      0.0163         &      0.0517         &      0.0703\sym{***}&      0.0117         \\
                    &      (4.30)         &      (2.28)         &      (0.06)         &     (-0.23)         &     (-1.01)         &      (0.56)         &      (0.84)         &      (1.85)         &      (5.40)         &      (1.92)         \\
\addlinespace
Constant            &       0.192\sym{***}&      0.0140\sym{***}&     0.00935\sym{***}&      0.0180\sym{***}&     0.00334\sym{***}&       0.314\sym{***}&      0.0204\sym{***}&     0.00734\sym{***}&      0.0407\sym{***}&     0.00367\sym{**} \\
                    &     (15.43)         &      (6.61)         &      (6.43)         &      (5.32)         &      (4.73)         &      (7.65)         &      (5.32)         &      (7.04)         &      (5.71)         &      (2.66)         \\
\midrule
Observations        &       29819         &       29819         &       29819         &       29819         &       29819         &       29819         &       29819         &       29819         &       29819         &       29819         \\
\midrule
Clustered SE & Yes & Yes & Yes & Yes & Yes & Yes & Yes & Yes & Yes & Yes \\ 
\bottomrule
\multicolumn{11}{l}{\footnotesize \textit{t} statistics in parentheses}\\
\multicolumn{11}{l}{\footnotesize \sym{*} \(p<0.05\), \sym{**} \(p<0.01\), \sym{***} \(p<0.001\)}\\
\end{tabular}
\end{adjustbox}
\end{table}

At last, in \ref{mun_fe} we show the estimates of the DID model coefficients as we include observations from December 2019 and (i) muniicpality fixed effects, (ii) White-robust standard errors. 

\begin{table}[H]\centering
\def\sym#1{\ifmmode^{#1}\else\(^{#1}\)\fi}
\caption{DID estimates for \emph{Uncertainty} and \emph{Negative Sentiment}, municipality fixed effects (omitted), and clustered standard errors. \label{mun_fe}}
\begin{adjustbox}{max width=\textwidth}
\begin{tabular}{lrrrrrrrrrr}
\toprule
&\multicolumn{5}{c}{Uncertainty}&\multicolumn{5}{c}{Negative Sentiment}\\
\toprule
                    &\multicolumn{1}{c}{(1)}&\multicolumn{1}{c}{(2)}&\multicolumn{1}{c}{(3)}&\multicolumn{1}{c}{(4)}&\multicolumn{1}{c}{(5)}&\multicolumn{1}{c}{(6)}&\multicolumn{1}{c}{(7)}&\multicolumn{1}{c}{(8)}&\multicolumn{1}{c}{(9)}&\multicolumn{1}{c}{(10)}\\
                    &\multicolumn{1}{c}{All}&\multicolumn{1}{c}{Economics}&\multicolumn{1}{c}{Health}&\multicolumn{1}{c}{Politics}&\multicolumn{1}{c}{Lockdown Pol.}&\multicolumn{1}{c}{All}&\multicolumn{1}{c}{Economics}&\multicolumn{1}{c}{Health}&\multicolumn{1}{c}{Politics}&\multicolumn{1}{c}{Lockdown Pol.}\\
\midrule
post=1              &      0.0626\sym{***}&     0.00895\sym{***}&      0.0634\sym{***}&    0.000208         &      0.0201\sym{***}&     -0.0212         &    -0.00331         &      0.0364\sym{***}&    -0.00565         &     0.00561\sym{**} \\
                    &      (6.00)         &      (4.12)         &      (7.14)         &      (0.05)         &     (11.51)         &     (-0.66)         &     (-1.14)         &      (5.71)         &     (-1.00)         &      (2.63)         \\
\addlinespace
post=2              &      0.0717\sym{***}&      0.0152\sym{***}&      0.0713\sym{***}&   -0.000229         &      0.0195\sym{***}&     -0.0446         &     0.00212         &      0.0409\sym{***}&     -0.0146\sym{**} &     0.00732\sym{*}  \\
                    &      (5.75)         &      (4.91)         &      (9.14)         &     (-0.06)         &      (7.14)         &     (-1.62)         &      (0.58)         &      (6.75)         &     (-3.35)         &      (2.36)         \\
\addlinespace
zonarossa=1 $\times$ post=1&      0.0170         &     -0.0175\sym{*}  &      0.0265\sym{*}  &      0.0125\sym{*}  &     0.00494         &    0.000895         &     -0.0159         &      0.0456\sym{**} &      0.0409\sym{***}&      0.0133         \\
                    &      (0.16)         &     (-2.06)         &      (2.14)         &      (2.27)         &      (0.32)         &      (0.03)         &     (-1.82)         &      (3.31)         &      (5.68)         &      (1.19)         \\
\addlinespace
zonarossa=1 $\times$ post=2&     -0.0216         &     -0.0137         &    -0.00686         &     0.00208         &     -0.0122\sym{**} &      0.0259         &    -0.00577         &      0.0520         &      0.0638\sym{***}&    0.000967         \\
                    &     (-0.37)         &     (-1.65)         &     (-0.25)         &      (0.36)         &     (-2.86)         &      (0.68)         &     (-0.39)         &      (1.77)         &      (4.67)         &      (0.21)         \\
\addlinespace
Constant            &       0.216\sym{***}&      0.0569\sym{***}&      0.0110         &    0.000128         &     -0.0161\sym{***}&       0.595\sym{***}&       0.109\sym{***}&       0.118\sym{***}&      0.0382\sym{***}&    -0.00579\sym{*}  \\
                    &     (22.39)         &     (23.89)         &      (1.68)         &      (0.04)         &     (-7.70)         &     (25.73)         &     (38.69)         &     (23.73)         &     (10.64)         &     (-2.42)         \\
\midrule
Observations        &       29819         &       29819         &       29819         &       29819         &       29819         &       29819         &       29819         &       29819         &       29819         &       29819         \\
\bottomrule
\multicolumn{11}{l}{\footnotesize \textit{t} statistics in parentheses}\\
\multicolumn{11}{l}{\footnotesize \sym{*} \(p<0.05\), \sym{**} \(p<0.01\), \sym{***} \(p<0.001\)}\\
\end{tabular}
\end{adjustbox}
\end{table}

\begin{table}[H]\centering
\def\sym#1{\ifmmode^{#1}\else\(^{#1}\)\fi}
\caption{DID Regression table for \emph{Uncertainty} and \emph{Negative Sentiment}, aggregated and grouped by topics, with White Standard Errors. \label{did_1}}
\begin{adjustbox}{max width=\textwidth}
\begin{tabular}{lrrrrrrrrrr}
\toprule
&\multicolumn{5}{c}{Uncertainty}&\multicolumn{5}{c}{Negative Sentiment}\\
\toprule
                    &\multicolumn{1}{c}{(1)}&\multicolumn{1}{c}{(2)}&\multicolumn{1}{c}{(3)}&\multicolumn{1}{c}{(4)}&\multicolumn{1}{c}{(5)}&\multicolumn{1}{c}{(6)}&\multicolumn{1}{c}{(7)}&\multicolumn{1}{c}{(8)}&\multicolumn{1}{c}{(9)}&\multicolumn{1}{c}{(10)}\\
                    &\multicolumn{1}{c}{All}&\multicolumn{1}{c}{Economics}&\multicolumn{1}{c}{Health}&\multicolumn{1}{c}{Politics}&\multicolumn{1}{c}{Lockdown Pol.}&\multicolumn{1}{c}{All}&\multicolumn{1}{c}{Economics}&\multicolumn{1}{c}{Health}&\multicolumn{1}{c}{Politics}&\multicolumn{1}{c}{Lockdown Pol.}\\
\midrule
zonarossa=1         &      0.0606\sym{*}  &      0.0139         &     0.00652         &     -0.0140\sym{**} &     0.00167         &       0.108\sym{***}&      0.0169         &     0.00193         &     -0.0420\sym{***}&    0.000269         \\
                    &      (2.54)         &      (1.55)         &      (1.02)         &     (-3.19)         &      (0.41)         &      (3.95)         &      (1.59)         &      (0.33)         &    (-10.66)         &      (0.07)         \\
\addlinespace
post=1              &      0.0545\sym{***}&     0.00705\sym{***}&      0.0610\sym{***}&    -0.00259         &      0.0195\sym{***}&     -0.0501\sym{***}&    -0.00726\sym{**} &      0.0317\sym{***}&     -0.0146\sym{***}&     0.00460\sym{***}\\
                    &      (8.37)         &      (3.45)         &     (24.00)         &     (-1.19)         &     (12.22)         &     (-6.68)         &     (-3.20)         &     (14.50)         &     (-4.65)         &      (3.49)         \\
\addlinespace
post=2              &      0.0673\sym{***}&      0.0139\sym{***}&      0.0695\sym{***}&    -0.00284         &      0.0188\sym{***}&     -0.0661\sym{***}&   -0.000719         &      0.0381\sym{***}&     -0.0229\sym{***}&     0.00673\sym{***}\\
                    &      (9.81)         &      (6.06)         &     (23.79)         &     (-1.26)         &     (10.96)         &     (-8.53)         &     (-0.29)         &     (15.29)         &     (-7.38)         &      (4.58)         \\
\addlinespace
zonarossa=1 $\times$ post=1&      0.0231         &     -0.0149         &      0.0320\sym{**} &      0.0153\sym{*}  &     0.00300         &     0.00789         &     -0.0109         &      0.0521\sym{***}&      0.0507\sym{***}&      0.0124         \\
                    &      (0.81)         &     (-1.46)         &      (2.61)         &      (2.41)         &      (0.43)         &      (0.25)         &     (-0.93)         &      (4.57)         &      (6.64)         &      (1.92)         \\
\addlinespace
zonarossa=1 $\times$ post=2&     -0.0248         &     -0.0132         &     -0.0142         &     0.00612         &    -0.00883         &      0.0510         &     0.00131         &      0.0424\sym{**} &      0.0717\sym{***}&     0.00777         \\
                    &     (-0.76)         &     (-1.09)         &     (-1.02)         &      (0.96)         &     (-1.21)         &      (1.40)         &      (0.09)         &      (2.83)         &      (6.35)         &      (0.98)         \\
\addlinespace
Constant            &       0.195\sym{***}&      0.0145\sym{***}&     0.00768\sym{***}&      0.0197\sym{***}&     0.00402\sym{***}&       0.347\sym{***}&      0.0229\sym{***}&     0.00943\sym{***}&      0.0449\sym{***}&     0.00541\sym{***}\\
                    &     (37.25)         &      (9.18)         &      (6.66)         &     (10.74)         &      (4.81)         &     (55.13)         &     (11.58)         &      (7.38)         &     (16.40)         &      (5.58)         \\
\midrule
Observations        &       29819         &       29819         &       29819         &       29819         &       29819         &       29819         &       29819         &       29819         &       29819         &       29819         \\
\bottomrule
\multicolumn{11}{l}{\footnotesize \textit{t} statistics in parentheses}\\
\multicolumn{11}{l}{\footnotesize \sym{*} \(p<0.05\), \sym{**} \(p<0.01\), \sym{***} \(p<0.001\)}\\
\end{tabular}
\end{adjustbox}
\end{table}

\end{document}
