# Supplementary material for: Breaking Down the Lockdown: The Causal Effects of Stay-At-Home Mandates on Uncertainty and Sentiments During the COVID-19 Pandemic
Source: arXiv:2212.01705 source file (2023-06-01)
Supplement: Supplementary file 2 [file excess_mortality_trends.tex]

\documentclass[../main.tex]{subfiles}
\begin{document}
To further assess the hypothesis of quasi-randomized allocation of the lockdown, we test the differences between the red and orange zone with respect to both the underlying rate of contagion and their observable characteristics, whereas the lack of difference does support its random allocation. We start by looking at the (unobserved) rate of COVID-19 contagion by retrieving it from the (observed) excess mortality of 2020 with respect to the previous five years (2015-2019).\footnote{We refer to \textcite{manski2021estimating} on the usage of excess mortality to derive the underlying contagion rates in the absence of reliable testing data. Please note that here we use excess mortality as a proxy of the contagion rate assuming that the mortality rates between the red and orange zone are highly similar. This seems plausible given the similar demographic characteristics in the two areas (see Appendix section \ref{}).} Then, we check the pre-treatment demographic and socio-economic characteristics. The results of these tests are reported in Appendix section \ref{}. No statistically detectable differences are found. Since the underlying contagion rate in the red and orange zone can be assumed the same, the treatment represents, thus, the only difference between the two areas.

Given that the scope of testing was very limited at the beginning of the pandemic, we look at excess mortality, which is a good proxy for the underlying contagion. In Figure \ref{fig:mov_avg_mort}, we compare the 14-days moving average for mortality in the years 2015-2019 (green) and 2020 (gold). Panel (a) displays the results for the red zone, panel (b) for the orange zone. The figure shows that there are no noticeable differences in the mortality rates in the pre-lockdown trends between the red zone and the orange zone municipalities. This result suggests that the spread and the fatality rate of COVID-19 was similar in the two zones. Figures \ref{fig:mov_avg_mort_diff}-\ref{fig:mov_avg_mort_diff_cumsum} further corroborate this evidence.\footnote{Figure \ref{fig:mov_avg_mort_diff} simply shows the difference between the number of daily deaths in 2020 and the average daily death in 2015-2019 for the red and orange zones. Figure \ref{fig:mov_avg_mort_diff_smooth} does the same, but adds a smoothed model. Figure \ref{fig:mov_avg_mort_diff_cumsum} displays the cumulative trend in excess mortality.} The trends in excess mortality (measured as the difference between daily deaths recorded in 2020 and the average daily death in 2015-2019) was very similar in the two zones before the implementation of the lockdown measure. Against this backdrop, the geographical distribution of the lockdown policies that followed such discovery depended on the random discovery of the first patient, and not on the underlying diffusion of the virus.\footnote{We report the moving average for only the \emph{orange zone} municipalities featured in the analysis.} The randomness of the allocation of units to the treatment enables us to study the causal effect of lockdown policies on the uncertainty and sentiments of treated individuals.

\begin{figure}[!htb]
  \begin{subfigure}[h]{0.5\textwidth}
    \includegraphics[width=\textwidth]{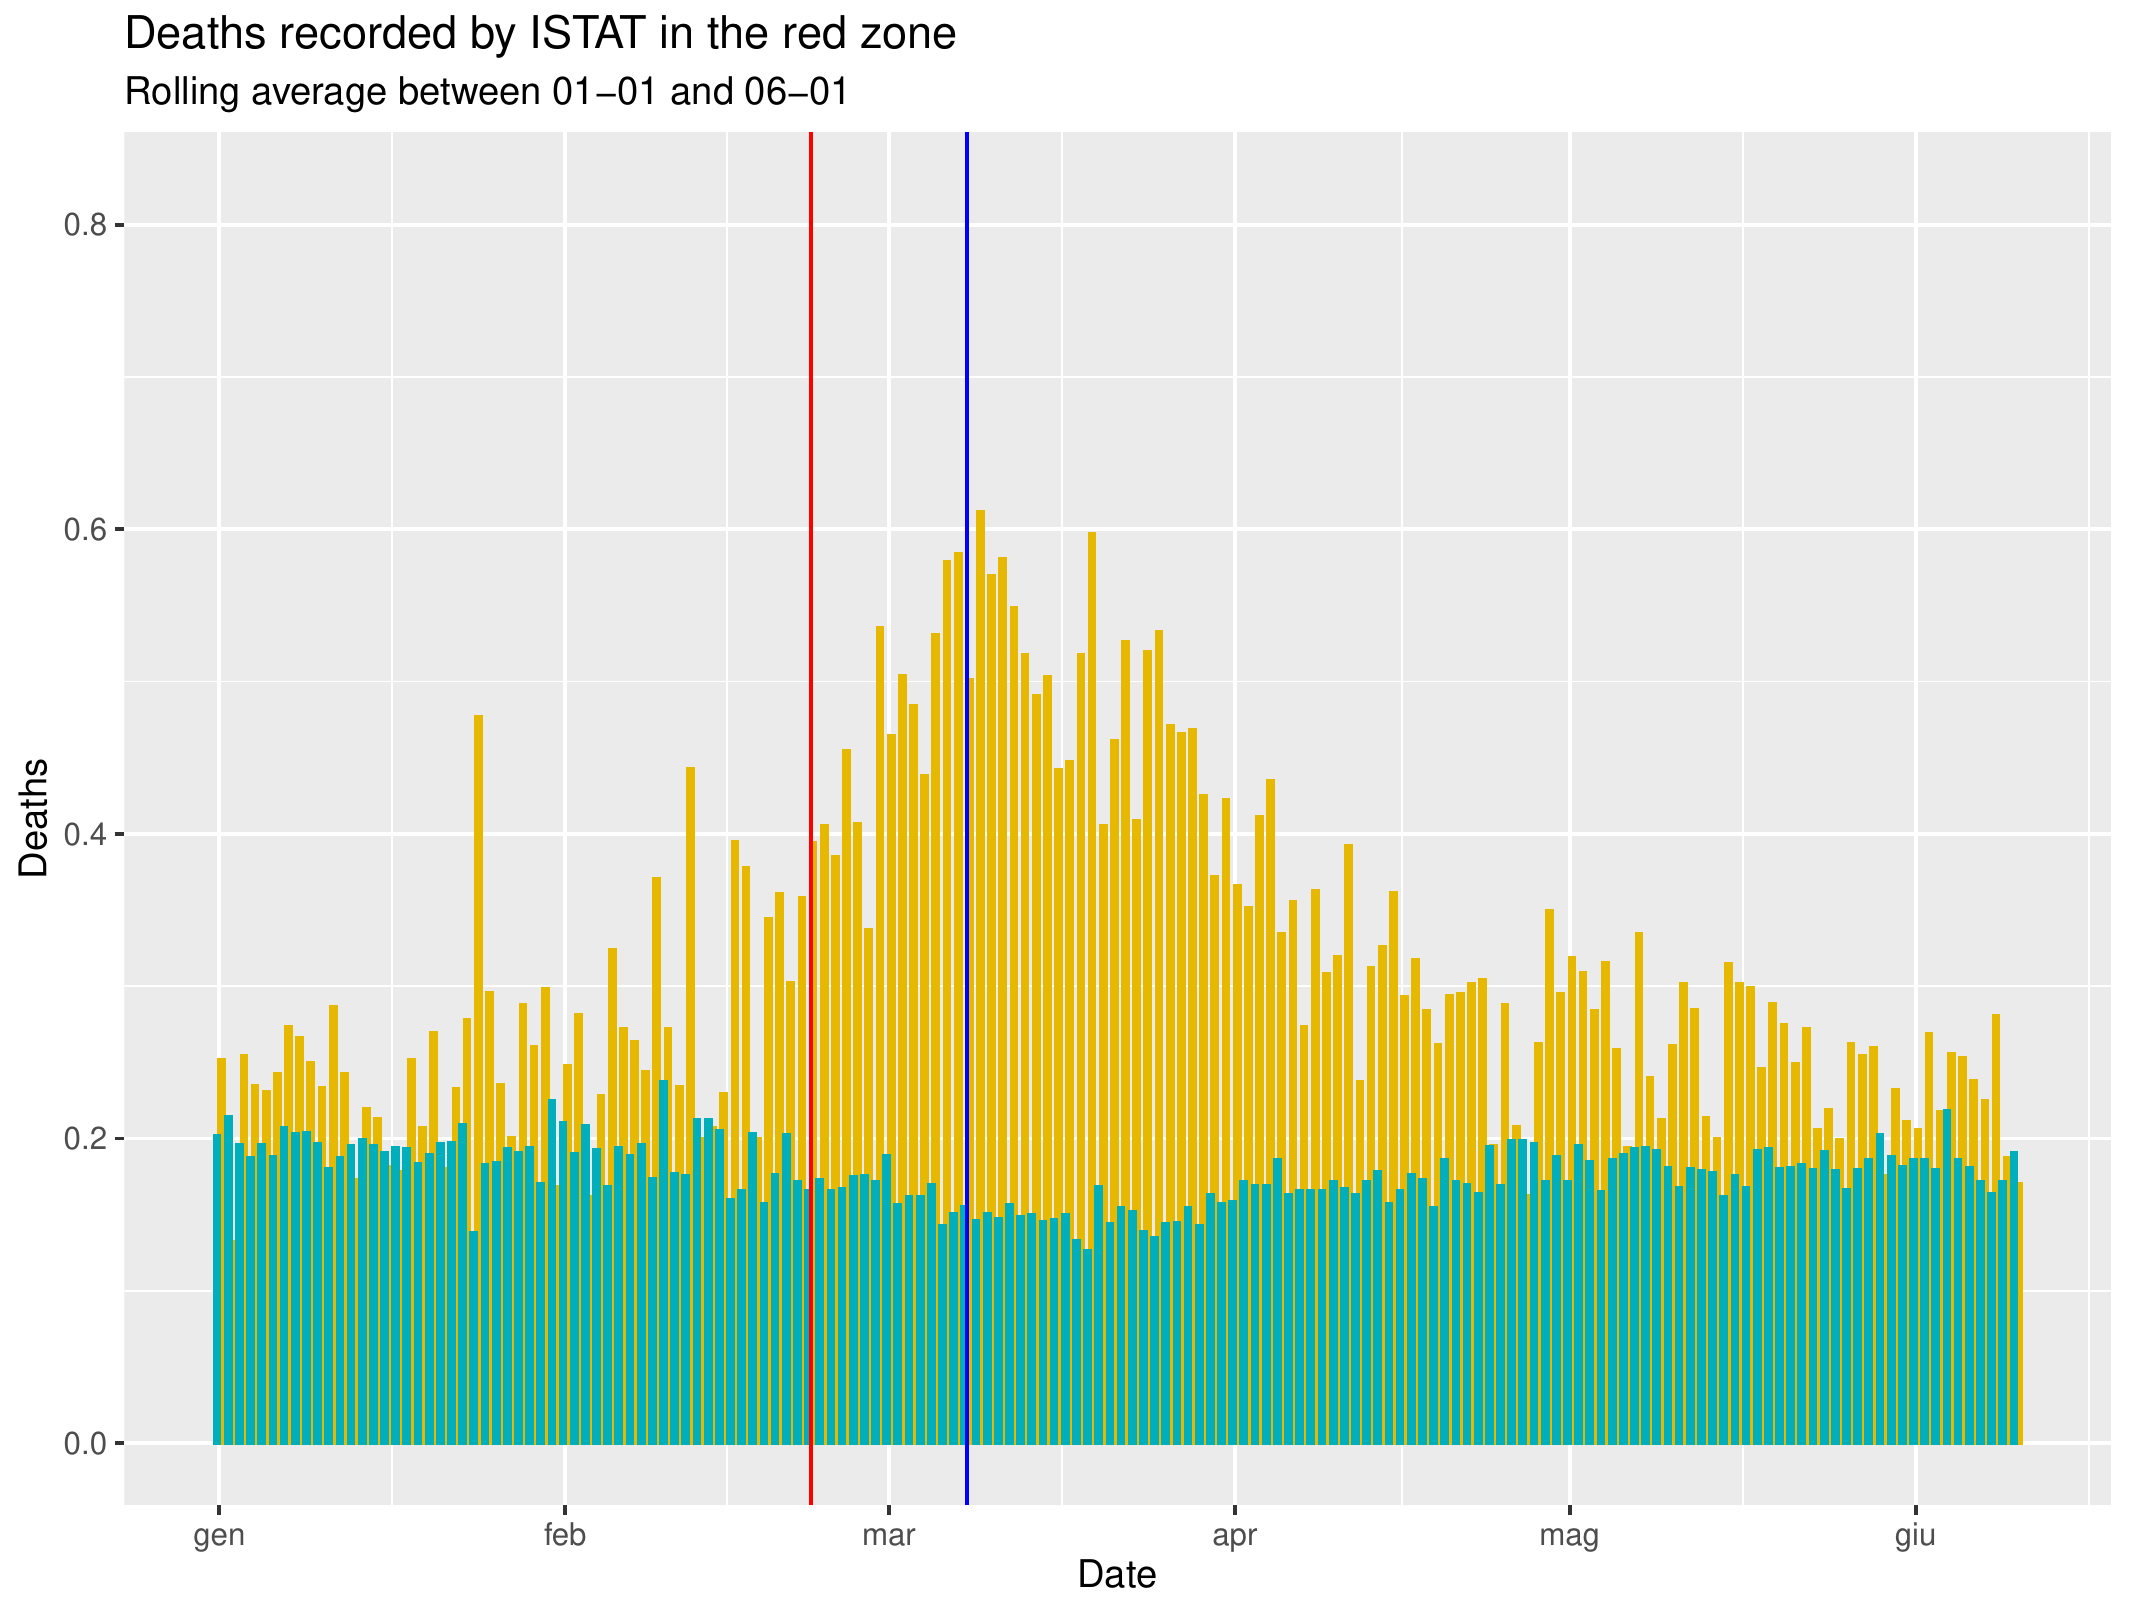}
   \caption{Red Zone}
    \label{fig:f3}
  \end{subfigure}
  \hfill
 \begin{subfigure}[h]{0.5\textwidth}
    \includegraphics[width=\textwidth]{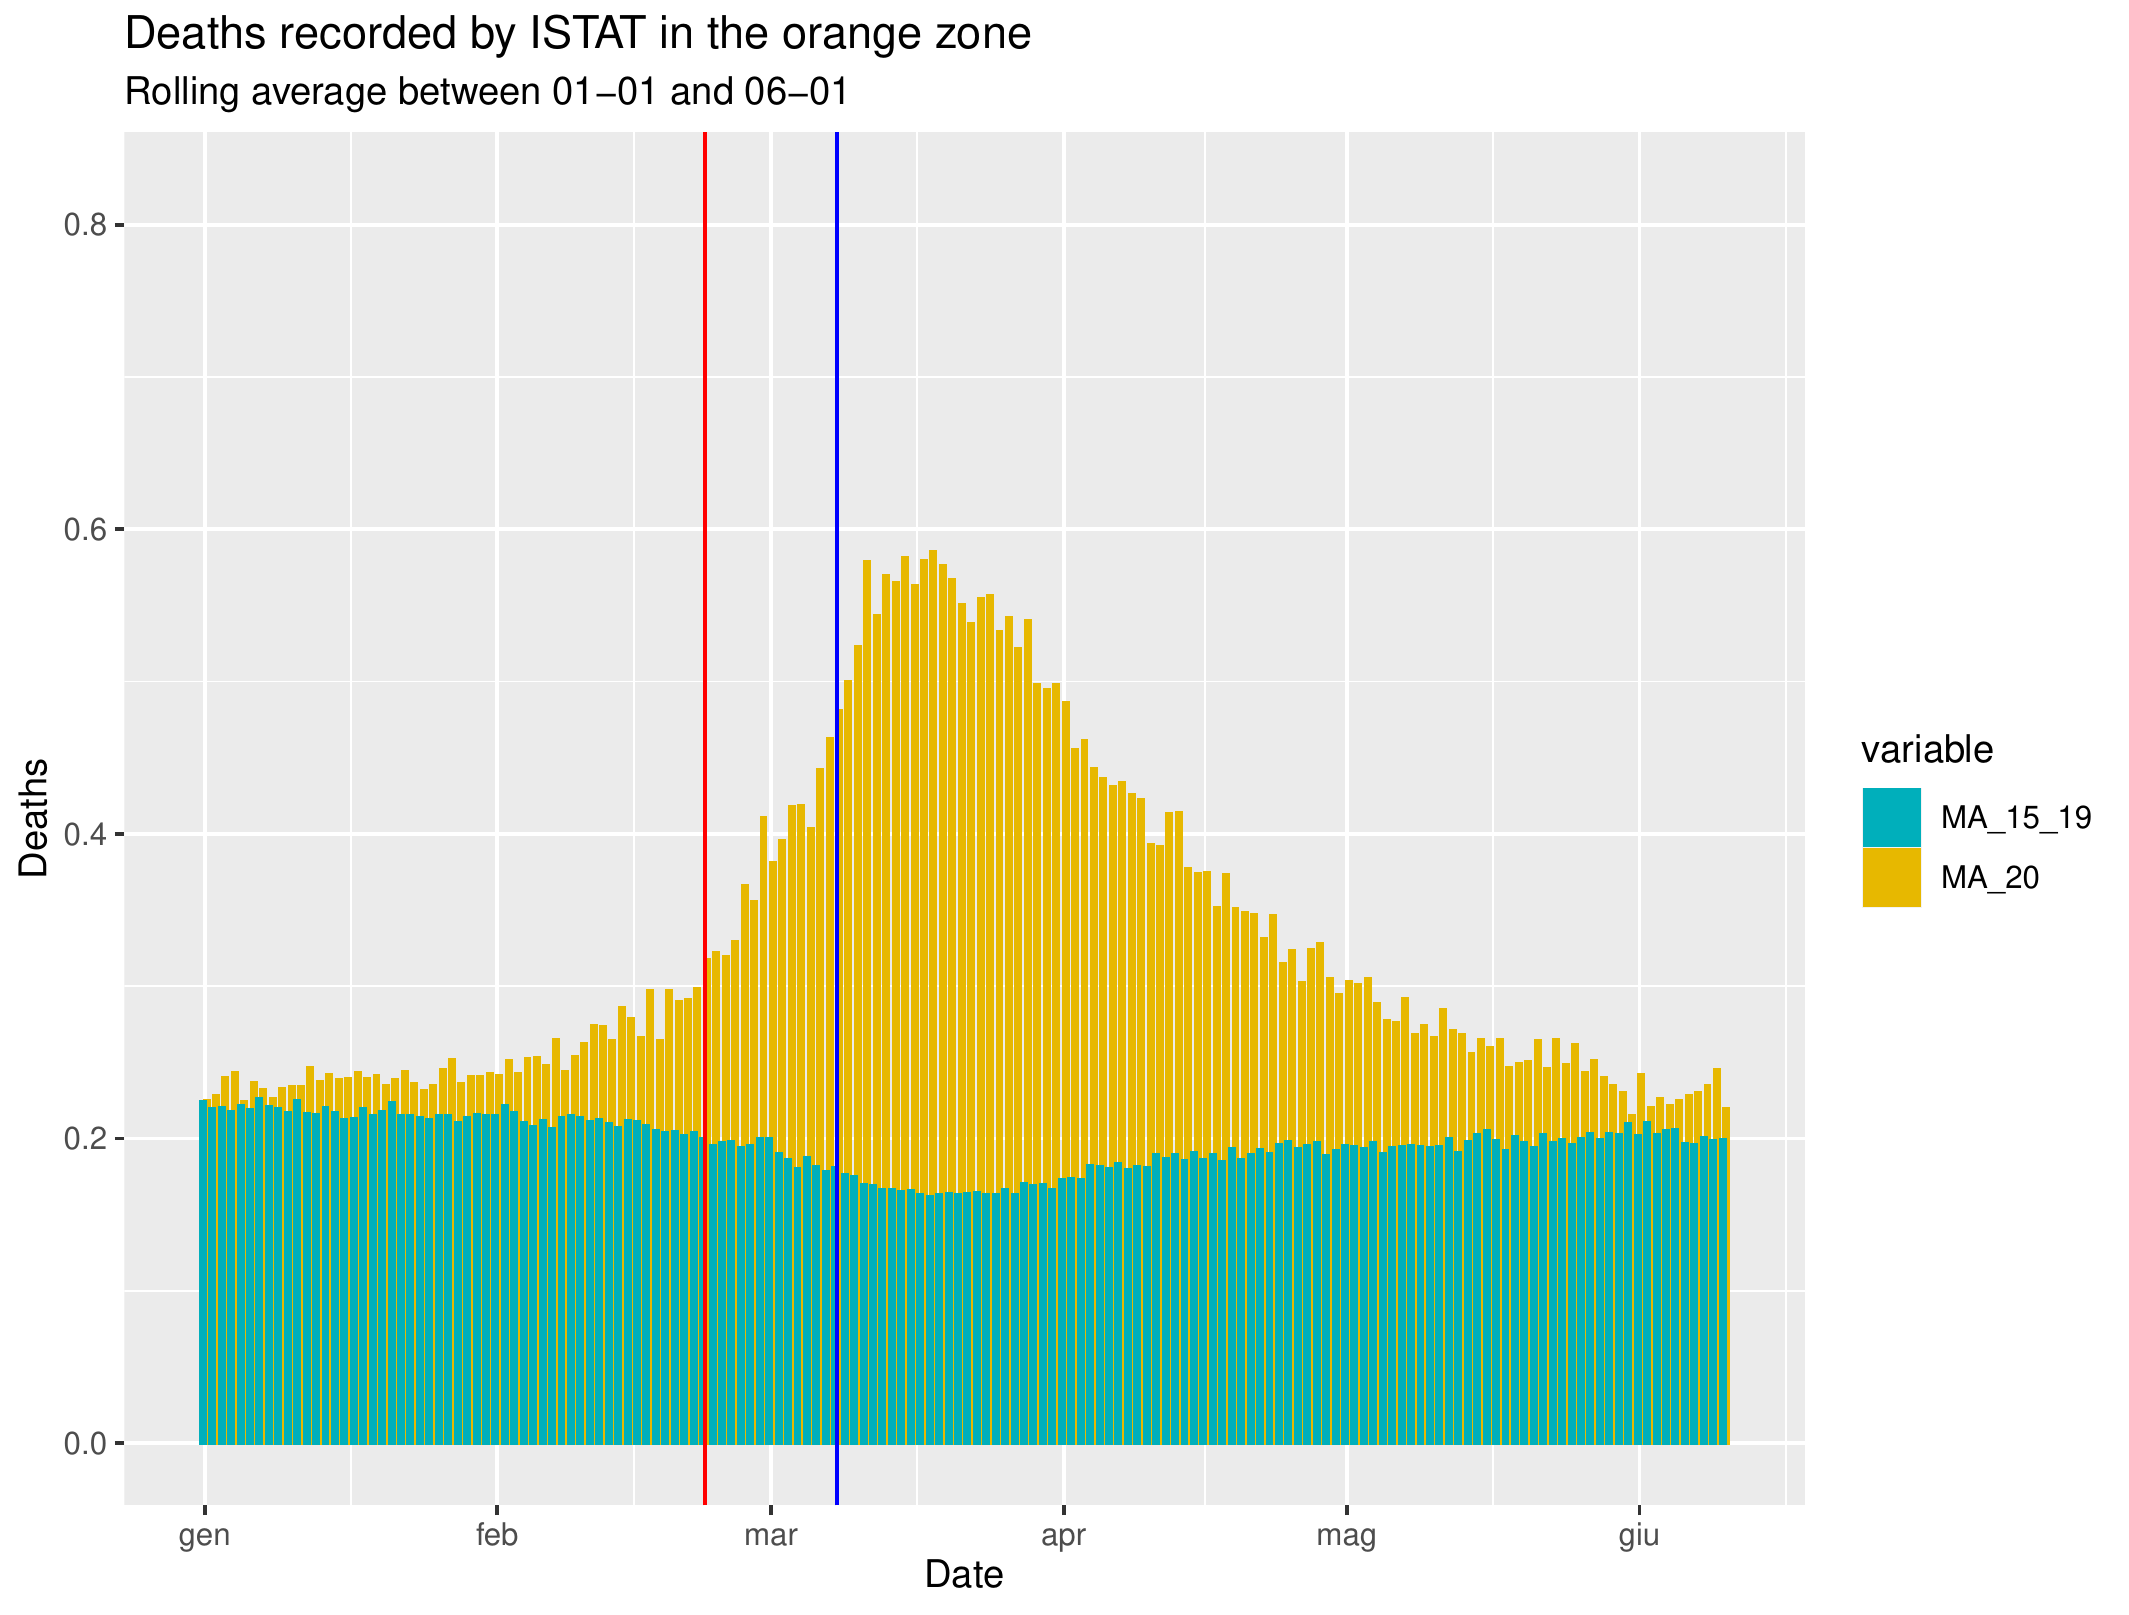}
    \caption{Orange Zone}
    \label{fig:f3}
  \end{subfigure}
  \caption{Fourteen days moving average for mortality in the years 2015-2019 (green) and 2020 (gold) in the red zone (a) vs excess mortality in the orange zone cities located within 42km from Codogno (319 municipalities) (b). The red vertical line indicates the date of the first lockdown, while the blue vertical line indicates the date of the extension of the lockdown to the entire national territory.}
  \label{fig:mov_avg_mort}
\end{figure}

\begin{figure}[H]
\centering
\includegraphics[scale = 0.5]{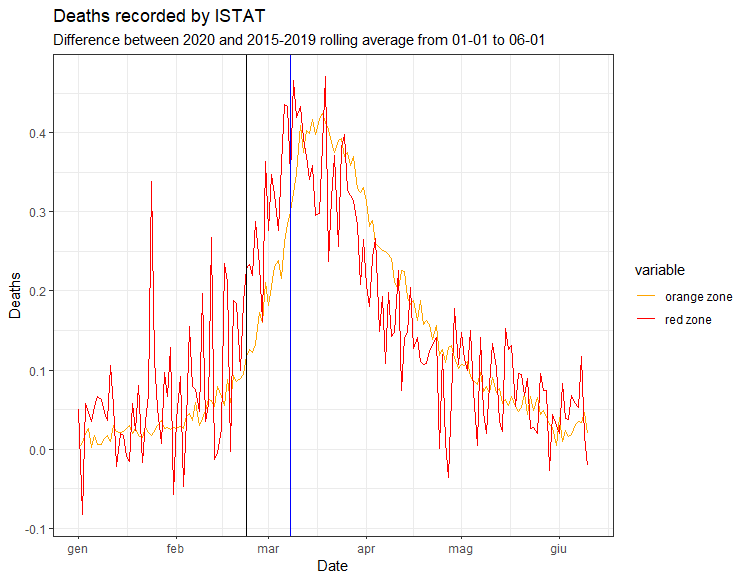}
  \caption{Difference in fourteen days moving average for mortality in the years 2015-2019 and 2020 in the red zone and in the orange zone cities located within 42km from Codogno (319 municipalities).}
  \label{fig:mov_avg_mort_diff}
\end{figure}

\begin{figure}[H]
\centering
\includegraphics[scale = 0.5]{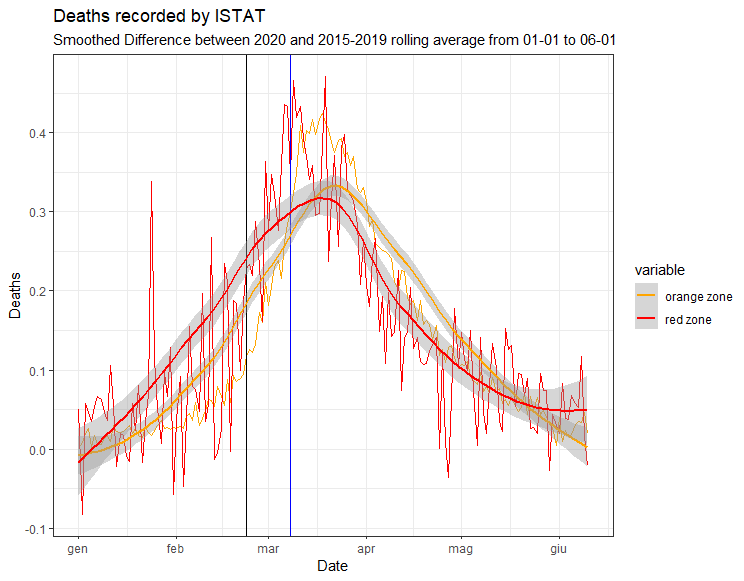}
  \caption{Smoothed time series for difference in fourteen days moving average for mortality in the years 2015-2019 and 2020 in the red zone and in the orange zone cities located within 42km from Codogno (319 municipalities).}
  \label{fig:mov_avg_mort_diff_smooth}
\end{figure}

% local smooth = Local Polynomial Regression Fitting. Fit a polynomial surface determined by one or more numerical predictors, using local fitting.
% formula used in smoothing function =  y ~ x

\begin{figure}[H]
\centering
\includegraphics[scale = 0.5]{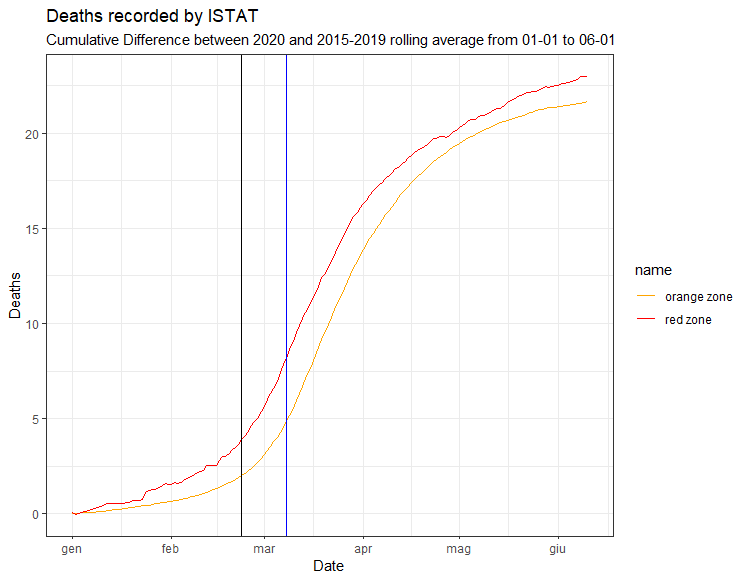}
\caption{Cumulative difference in fourteen days moving average for mortality in the years 2015-2019 and 2020 in the red zone and in the orange zone cities located within 42km from Codogno (319 municipalities).}
  \label{fig:mov_avg_mort_diff_cumsum}
\end{figure}

%% new mortality plots 

%Chi-Squred tests of independence:
Pearson's Chi-Squared tests of independence. The p-values are higher than 0\,05, we do not have sufficient evidence to reject the null hypothesis of independence between mortality in the red and orange zone. To avoid poor approximations of the p-values, we compute p-values by Monte Carlo simulation, with 2000 replicates used in the Monte Carlo test. 
\begin{table}[ht]
\caption{Chi-Squared tests of independence for difference in 14-days MA between (i) red zone and (ii) orange zone\label{cs_1}}
\centering
\begin{tabular}{rrrr}
  \hline
 Data & Statistic  & P-value \\ 
  \hline
 Diff MA 19-20  & 26082.00 & 0.00 \\ 
 Diff MA (divided by pop) 19-20 & 26082.00 & 0.00  \\
 Diff MA (divided by pop) 15/19-20 & 26082.00 & 0.00  \\ 
   \hline
\end{tabular}
\end{table}

\begin{table}[H]\centering
\def\sym#1{\ifmmode^{#1}\else\(^{#1}\)\fi}
\caption{Chi-Squared tests of independence for difference in 14-days MA of the months of January, February and March between (i) red zone and (ii) orange zone \label{cs_1}}
\begin{adjustbox}{max width=\textwidth}
\begin{tabular}{lrrrrrr}
\toprule 
\multicolumn{1}{c}{}&\multicolumn{2}{c}{\textbf{January}}&\multicolumn{2}{c}{\textbf{February}}\multicolumn{2}{c}{\textbf{March}}\\
\toprule
         &\multicolumn{1}{c}{Statistic}&\multicolumn{1}{c}{P-value}&\multicolumn{1}{c}{Statistic}&\multicolumn{1}{c}{P-value}&\multicolumn{1}{c}{Statistic}&\multicolumn{1}{c}{P-value}\\
\midrule
Diff MA 19-20 & 930.00 & 1.00 & 756.00 &  1.00  & 930.00  & 1.00  \\ 
Diff MA (divided by pop) 19-20 & 930.00 & 1.00 & 756.00  & 1.00 & 930.00 & 1.00\\
Diff MA (divided by pop) 15/19-20 & 930.00 & 1.00 & 756.00  & 1.00 & 930.00 & 1.00 \\
\bottomrule
\end{tabular}
\end{adjustbox}
\end{table}

\begin{figure}[H]
\centering
\includegraphics[scale = 0.5]{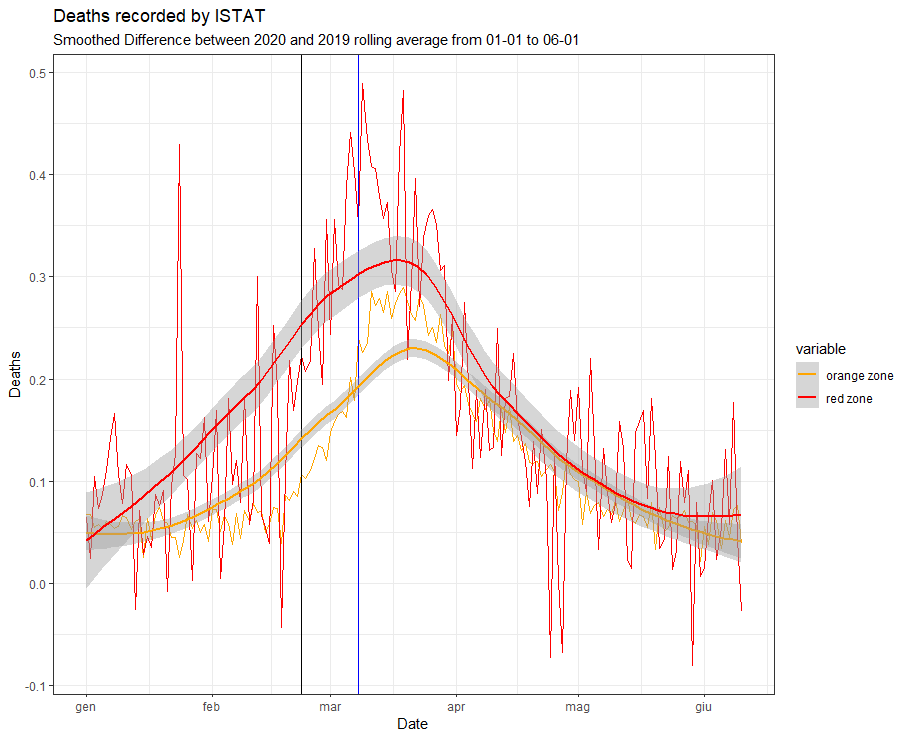}
\caption{Difference in fourteen days moving average for mortality in the years 2019 and 2020 in the red zone and in the orange zone cities located within 42km from Codogno (319 municipalities).}
  \label{fig:mov_avg_mort_diff_19_20}
\end{figure}

\begin{figure}[H]
\centering
\includegraphics[scale = 0.5]{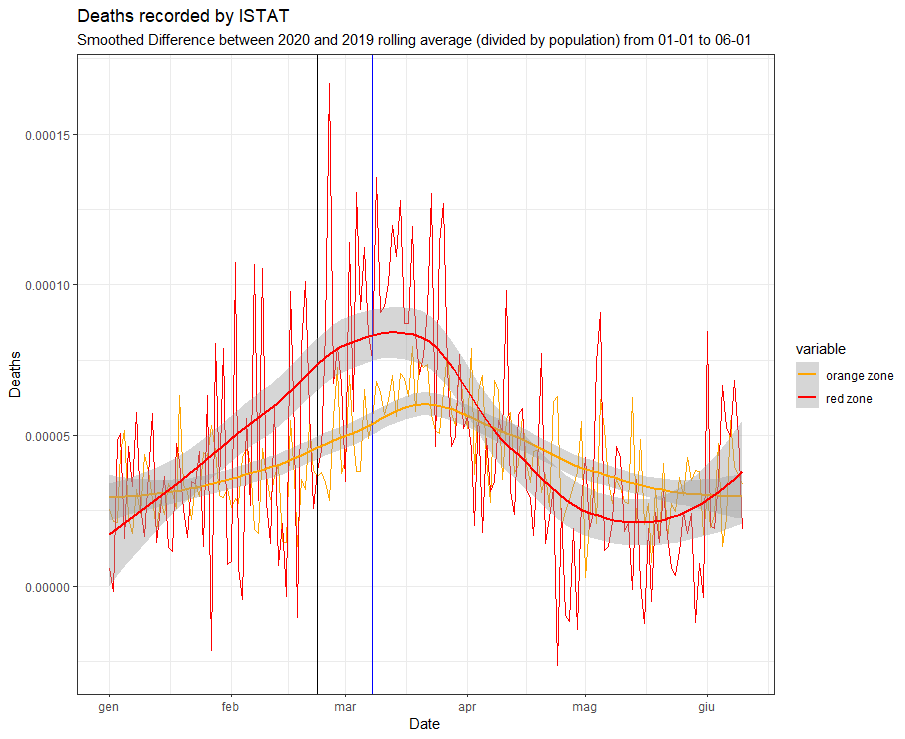}
\caption{Difference in fourteen days moving average for mortality in the years 2019 and 2020 (divided by population of 2019 and 2020) in the red zone and in the orange zone cities located within 42km from Codogno (319 municipalities).}
  \label{fig:mov_avg_mort_diff_19_20_pop_city}
\end{figure}

\begin{figure}[H]
\centering
\includegraphics[scale = 0.5]{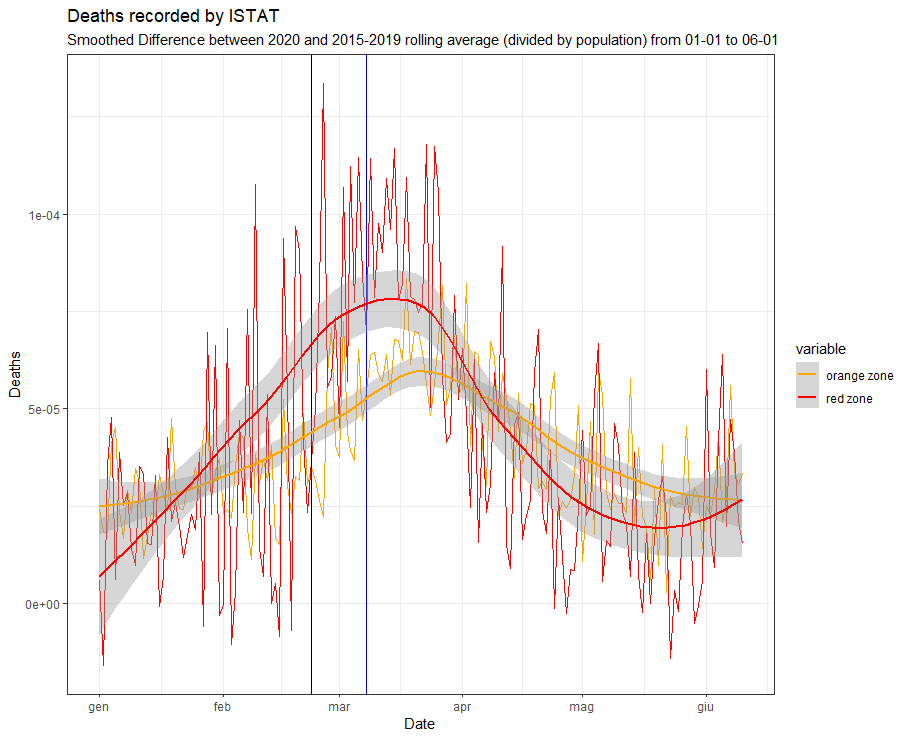}
\caption{Difference in fourteen days moving average for mortality in the years 2015-2019 and 2020 (divided by population of 2019 and 2020) in the red zone and in the orange zone cities located within 42km from Codogno (319 municipalities).}
  \label{fig:mov_avg_mort_diff_1519_20_pop_city}
\end{figure}

\end{document}
