# Supplementary material for: Breaking Down the Lockdown: The Causal Effects of Stay-At-Home Mandates on Uncertainty and Sentiments During the COVID-19 Pandemic
Source: arXiv:2212.01705 source file (2023-06-01)
Supplement: Supplementary file 3 [file descriptive_stats.tex]

\documentclass[../main.tex]{subfiles}
\begin{document}
\section{Descriptive Statistics}

In Figure \ref{fig:ds_1}, we report the sample estimates of the mean share of tweets expressing uncertainty and negative sentiment, along with with 95\% confidence intervals. The statistics are computed separately for the treatment (red zone), the control (orange zone).
%and by aggregating data from the larger sample of tweets accounting for observations from all Italy (excluding the red zone and orange zone cities), so that we can compare the national trend with that observed in the red and orange zones. 
For each group, we show the evolution of public opinion over pre-post-post periods, indicated with the labels 0, 1, and 2 respectively, marking the time of the enactment of the first lockdown measures at the local level and the later extension at the national level. 

Figure \ref{fig:ds_1a} shows that treated units display higher uncertainty than controls before the implementation of the restriction measures, but the difference between the two groups becomes less clearly significant as the lockdown policy is extended to the entire nation. 
%The share of uncertainty at the national level decreases over time, but it remains well above the share estimated for all other groups, even as the measures become nation-wide. Moreover, the trend among control units increases over time, differently from what is depicted at the national level. 
In Figure \ref{fig:ds_1b}, until the lockdown policy of the 23rd is implemented, there is no notable difference in mean shares of negative sentiment tweets between the red and the orange zone. After the treatment, the red zone expresses higher discontent, which will not matched again by controls once the policy becomes nation-wide. 
%At the aggregated level, the public opinion is more likely to express negative sentiments when posting online with respect to treated and controls, at least until the expansion of the measures at the national level.
\begin{figure}[H]
  \begin{subfigure}[h]{0.4\textwidth}
    \includegraphics[width=\textwidth]{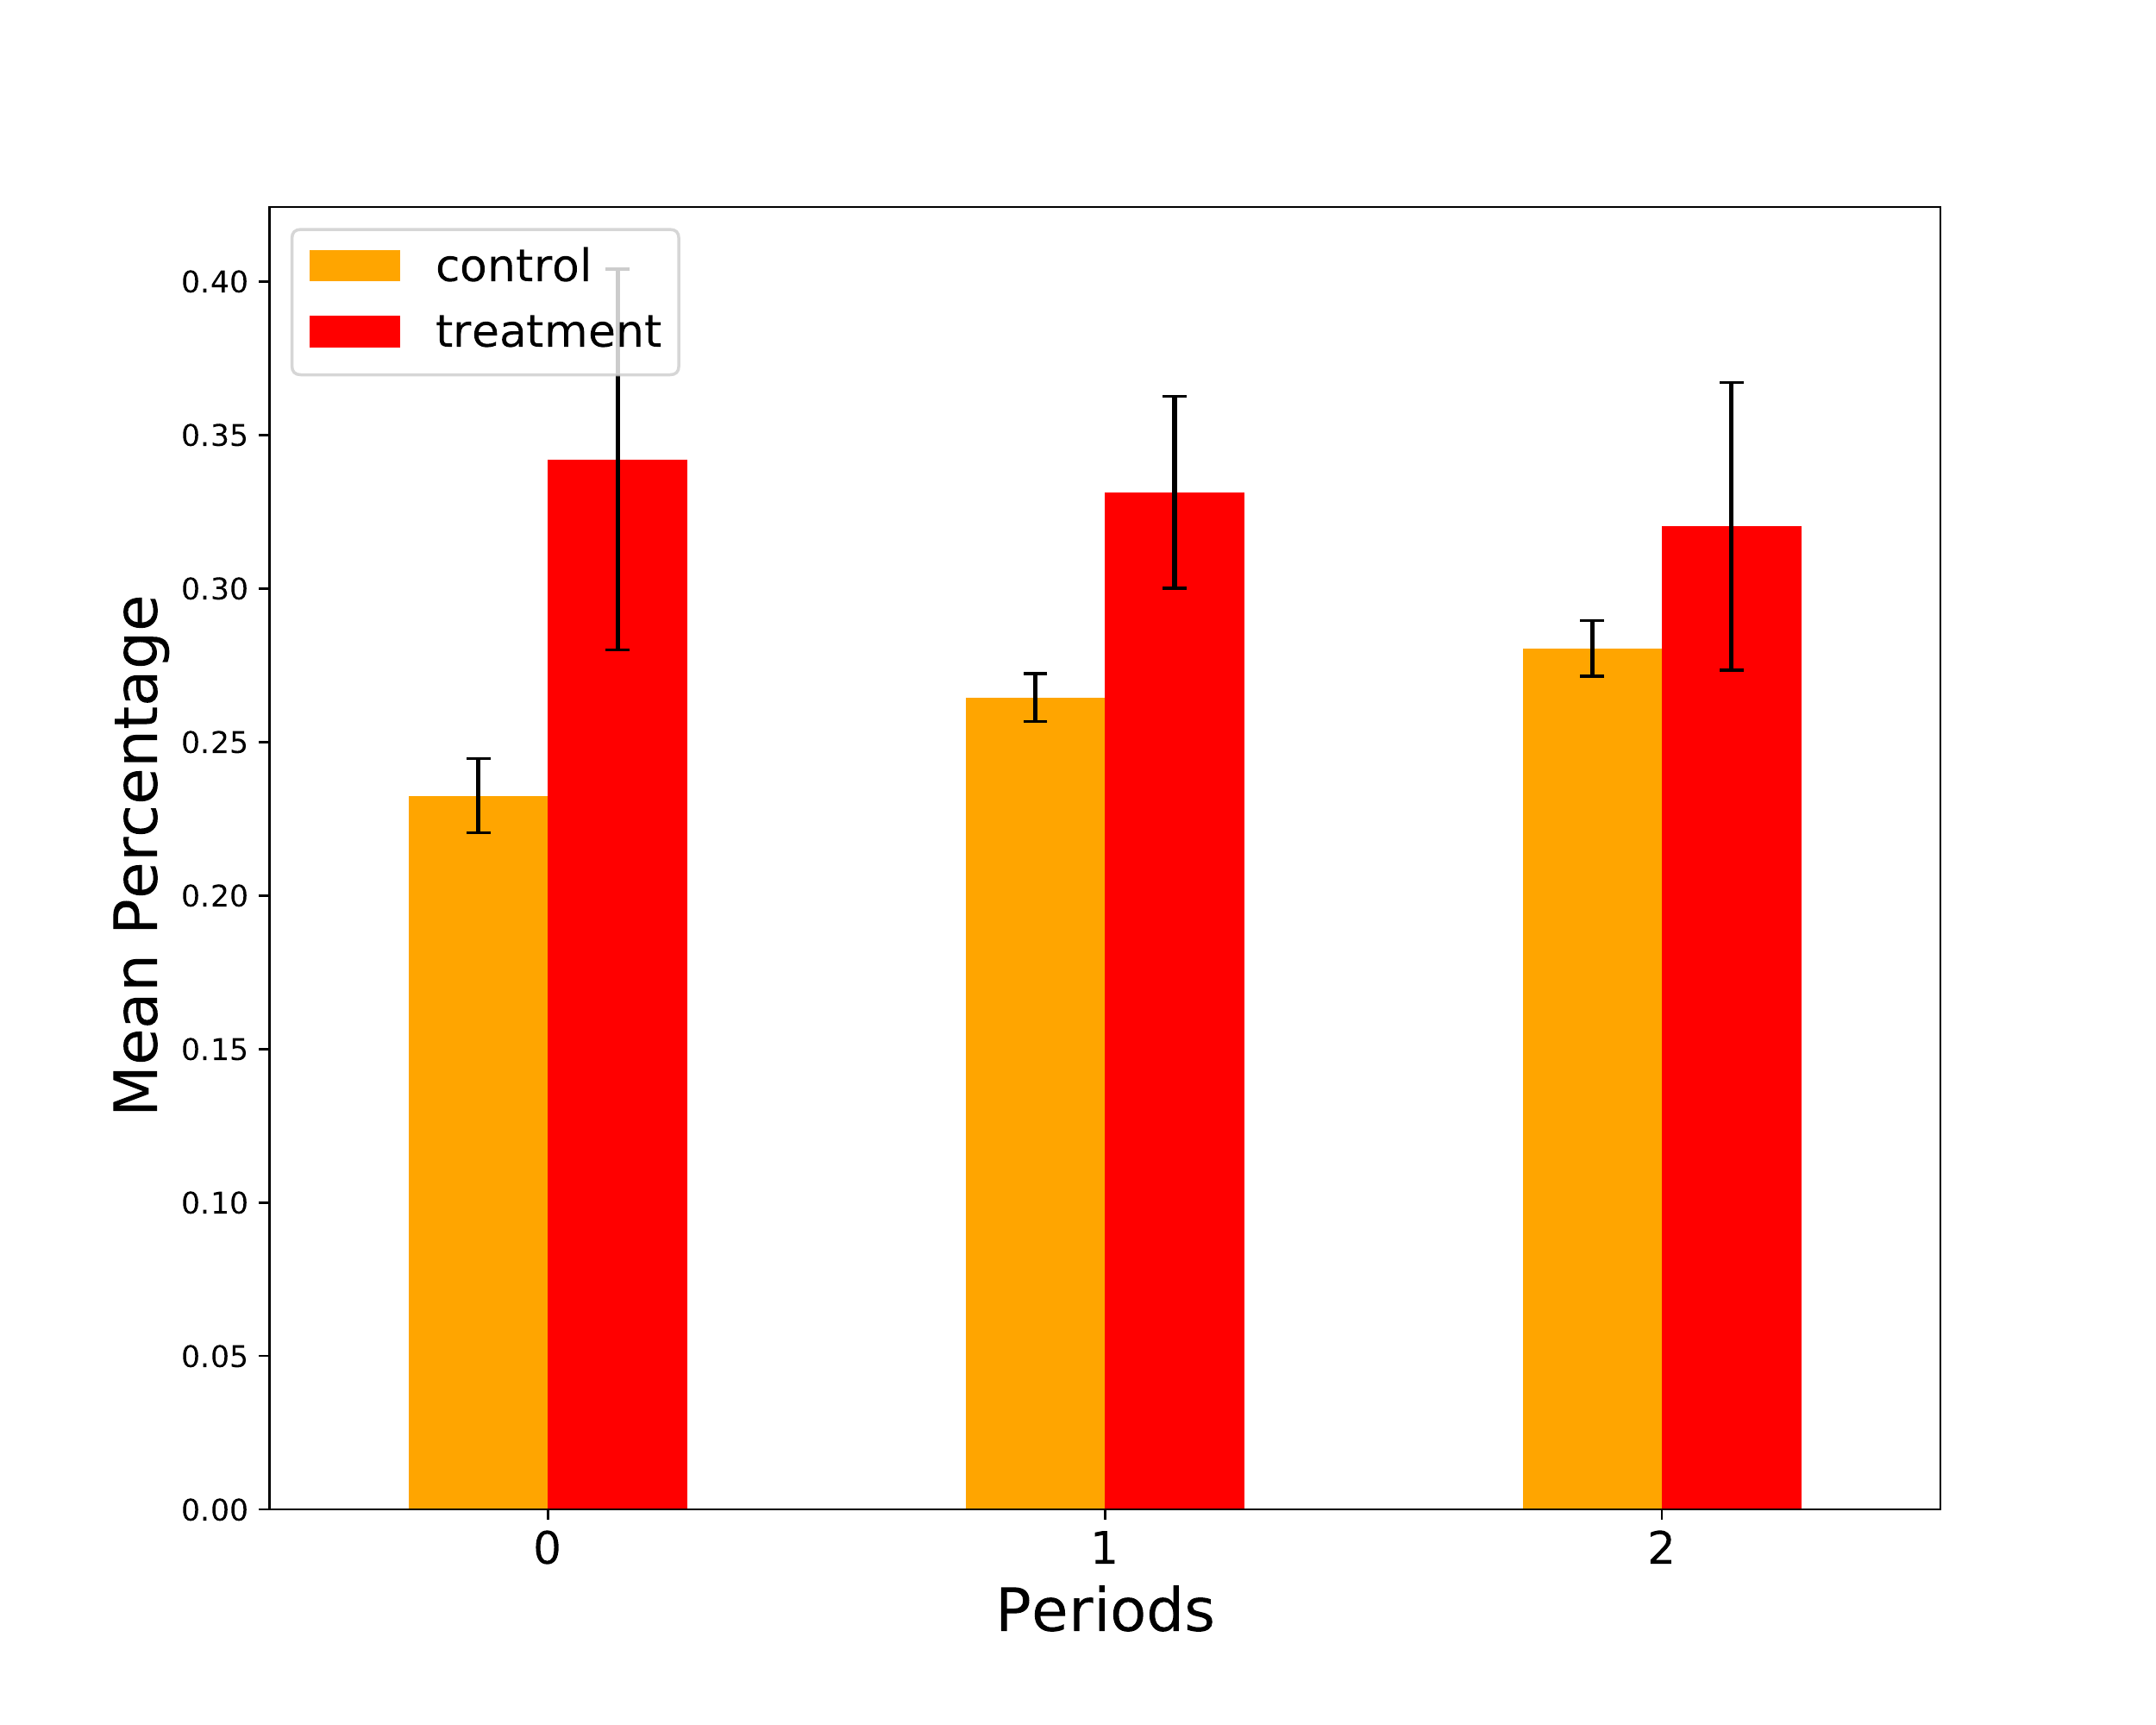}
    \caption{Uncertainty}
    \label{fig:ds_1a}
  \end{subfigure}
  \hfill
 \begin{subfigure}[h]{0.4\textwidth}
    \includegraphics[width=\textwidth]{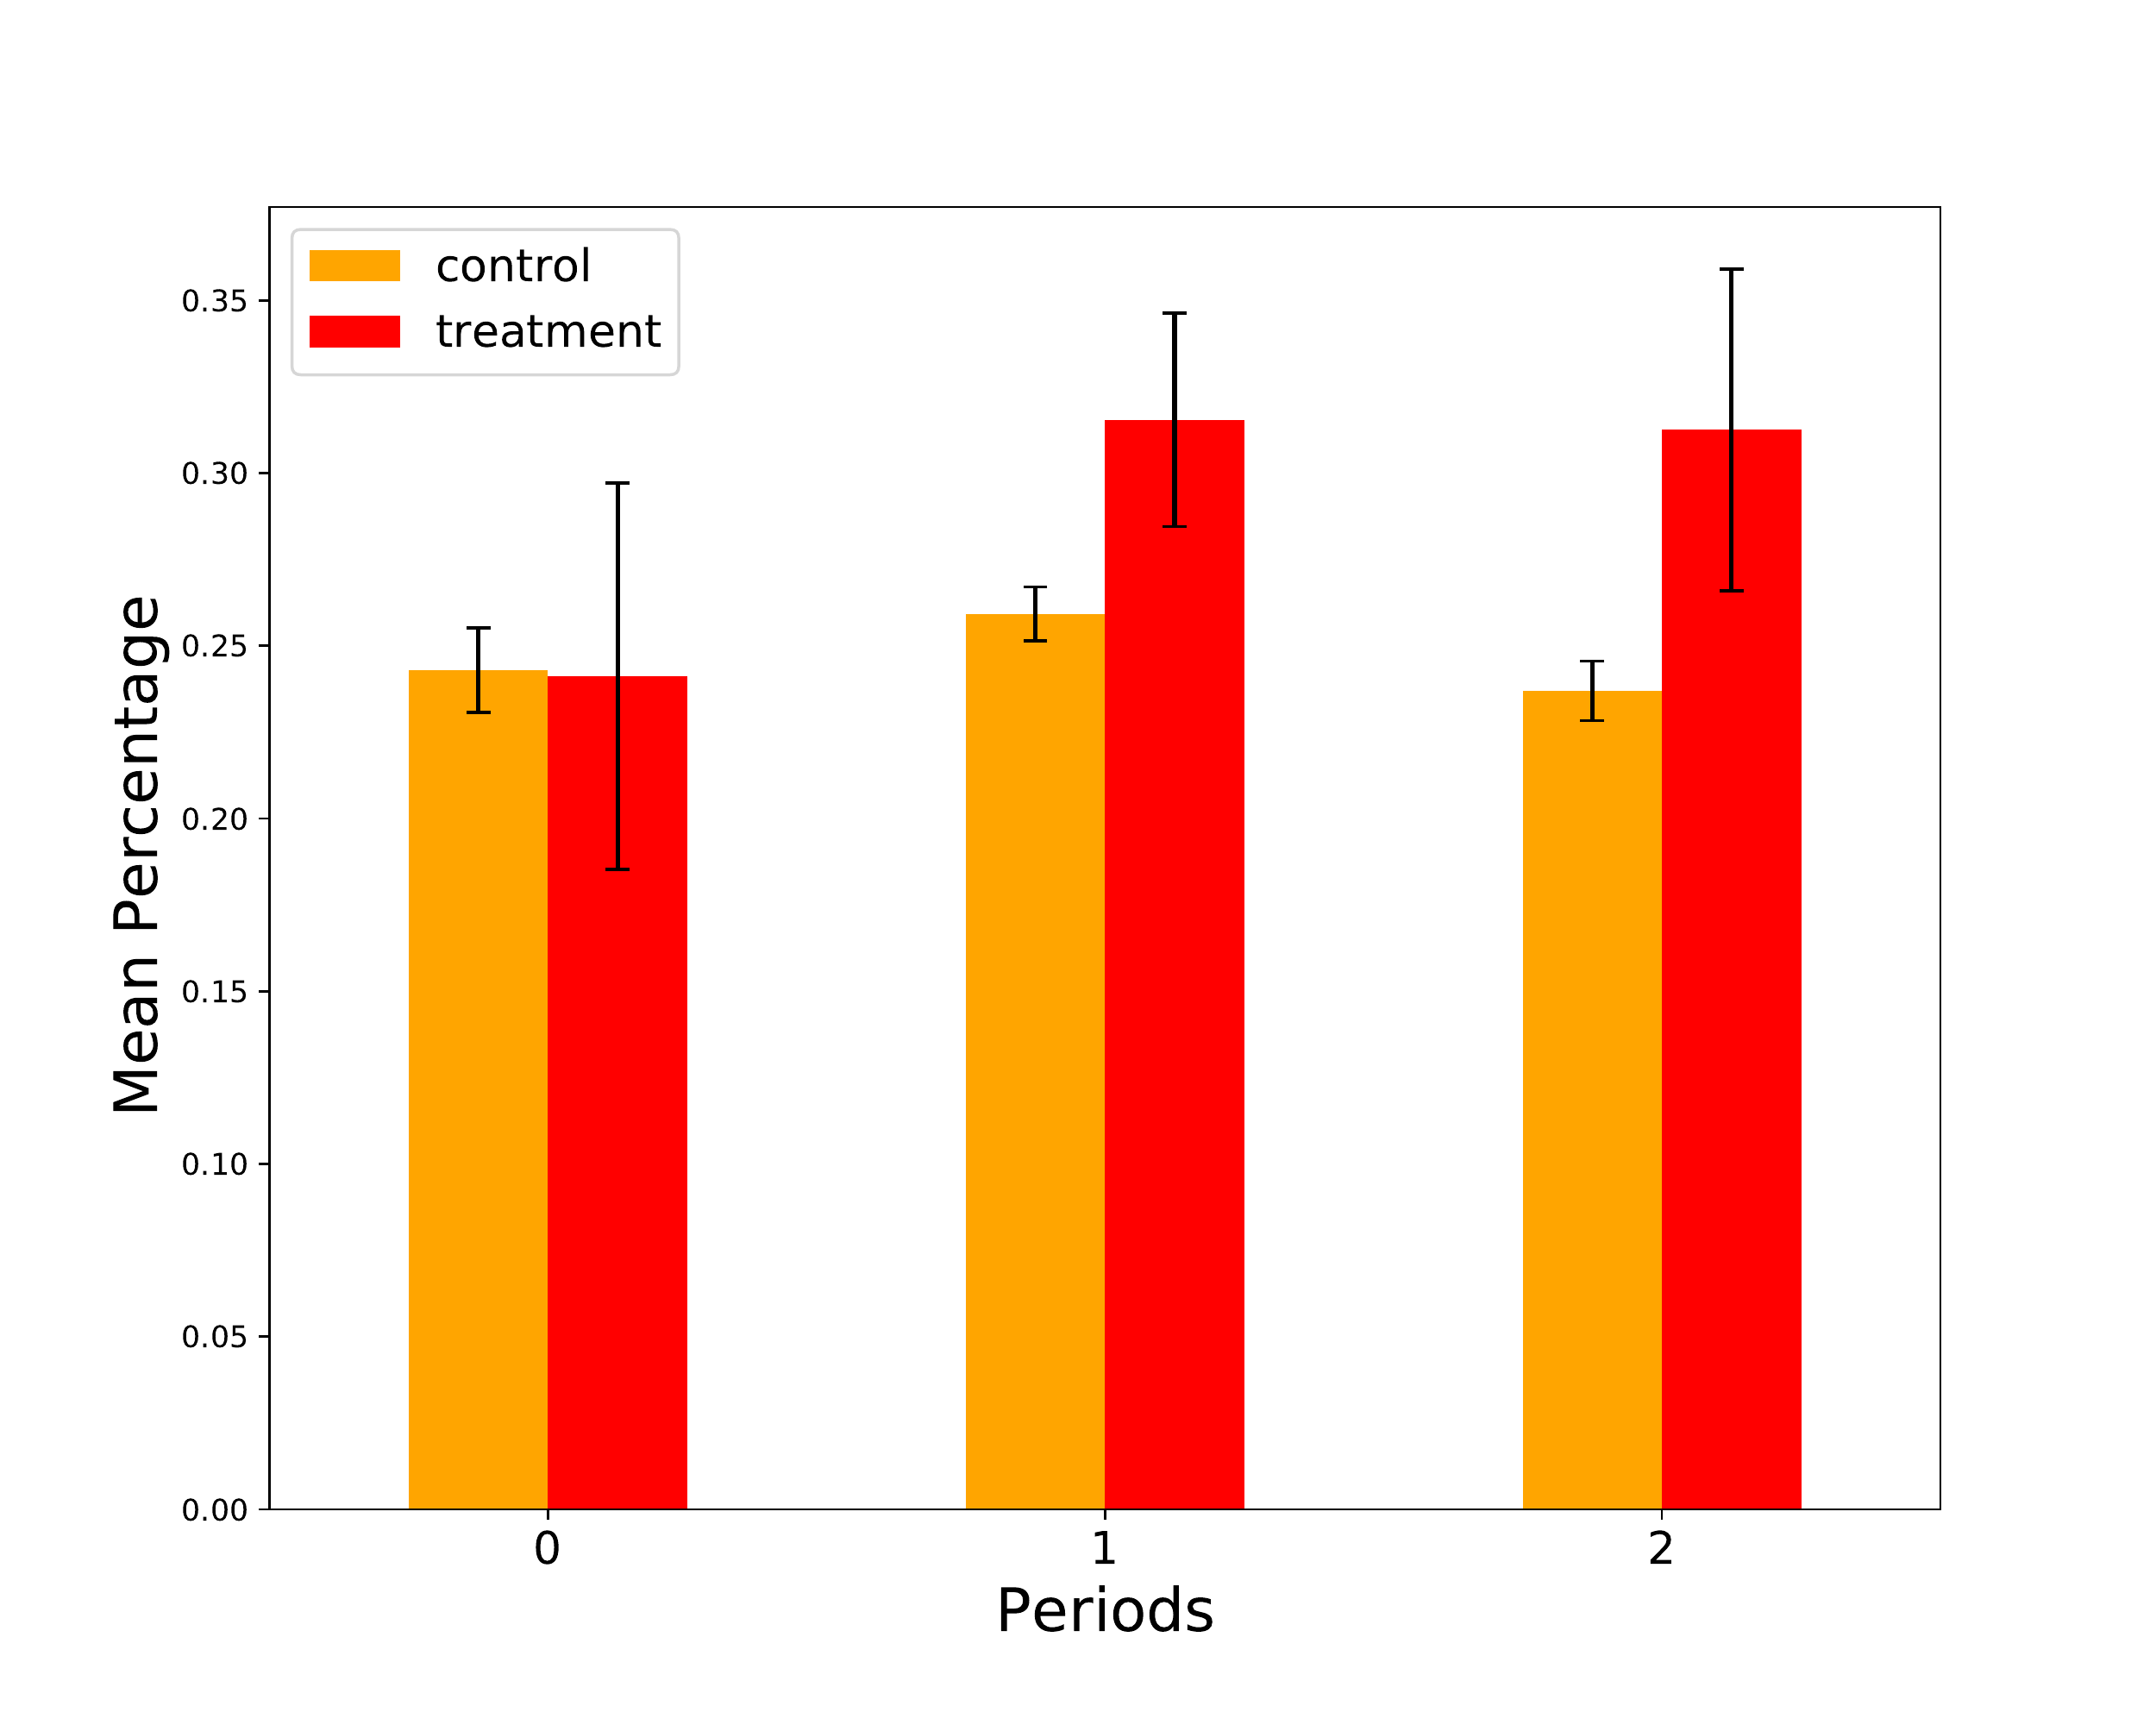}
    \caption{Negative Sentiment}
    \label{fig:ds_1b}
  \end{subfigure}
  \caption{Share of tweets classified as \emph{Uncertainty} and \emph{Negative sentiment} for \emph{control} and \emph{treated} cities.}
  \label{fig:ds_1}
\end{figure}
 
Figure \ref{fig:ds_2} reports the evolution over time of mean shares of uncertainty and negative sentiment tweets grouped by related topic. In Figure \ref{fig:ds_2a}, uncertainty expressed by economic-related tweets from the red zone seem to be decreasing after the measures are first enacted, while the trend among control units is increasing. No evident significant difference between treatment and control can be found over the time periods.

The first lockdown policy in the red zone is associated with a higher estimated share of health-related uncertain tweets than in the neighbouring cites of the orange zone, but the difference seems to be mitigated by the extension of the measures nation-wide (Figure \ref{fig:ds_2b}). 
%The aggregated data follows a decreasing trend with an estimated mean much higher than in the two other groups. 
Figure \ref{fig:ds_2c} shows no notable difference between treated and control units over the three time periods. 
%Uncertainty in politics discussions is decreasing at the aggregated level, while it seems to be slightly affected in the treated and control areas. 
In Figure \ref{fig:ds_2d}, the high share of uncertainty expressed by tweets related to the restrictions goes back to control levels at the beginning of the policy. On the contrary, control units display increasing preoccupation over the functioning of the lockdown policy. 
%Moreover, the share at the national level increases with the start of the first stay-at-home measures, but it soon decreases back to previous levels as the mandate is expanded nation-wide.  

In Figure \ref{fig:ds_3a}, the shares of tweets expressing dissatisfaction towards economic issues of the treated shows no evident difference with the control group. With the first lockdown policy, the sample mean is reduced for both treatment and control, albeit the variation is greater among the former. %At the aggregated level, negative sentiment tweets related to economics seem to be following an increasing trends, with an estimated sample mean way above the mean observed in both treated and control groups.
The mean share of health-related tweets expressing negative sentiment in the red zone is higher than the orange zone after the start of the first lockdown and the difference is maintained following the extension of the measures (Figure \ref{fig:ds_3b}). %Again, we see that negative feelings aggregated at national level are much more likely than among treated and controls. Also for politics-related tweets in Figure \ref{fig:ds_3c}, we see at the national level relatively high shares of negative emotions with a decreasing trend, a trend that is shared by the control group.
In Figure \ref{fig:ds_3c}, the sample mean among the treated is increasing over time, but still no notable dissimilarities are found with the control area. In Figure \ref{fig:ds_3d}, we see that negative emotions towards the lockdown policy follows an increasing trend in the control group. The beginning of the policy is associated with an small increase of dissatisfaction among the treated, and a slight decrease among controls, but no conclusion about any significant difference between the group means can be derived. 

%Some key facts seem to emerge when comparing the estimated trends among the three groups. At the aggregated level, the public opinion heavily relies on uncertainty and negative sentiments when posting online, a situation that is not reflected among the Lombard cities of the red and orange zones. The aggregated data seems to be generally following an opposite trend with respect to controls for many aspects of the public's debate. This suggests that the public opinion of those first subject to the lockdown policy differs from the \emph{vox-populi} emerging at the aggregate, national level. 
Considering only the stronger evidence supporting difference in means between treatment and control groups, the unexpected lockdown policy seems to be associated with higher shares of uncertainty and negative sentiment among the treated, with a lasting high share of discontent towards health-related issues for those subject to the restrictions.
%While the estimates of the share of uncertainty in tweets at the national level follow a decreasing trend, just as the treatment group in the red zone, the trend in negative sentiment instead is decreasing, in contrast with respect to the increasing share of discontent reported in the red zone, This suggests that the public opinion of those first subject to the lockdown policy differs from the \emph{vox-populi} emerging at the aggregate, national level. 

\begin{figure}[H]
  \begin{subfigure}[h]{0.4\textwidth}
    \includegraphics[width=\textwidth]{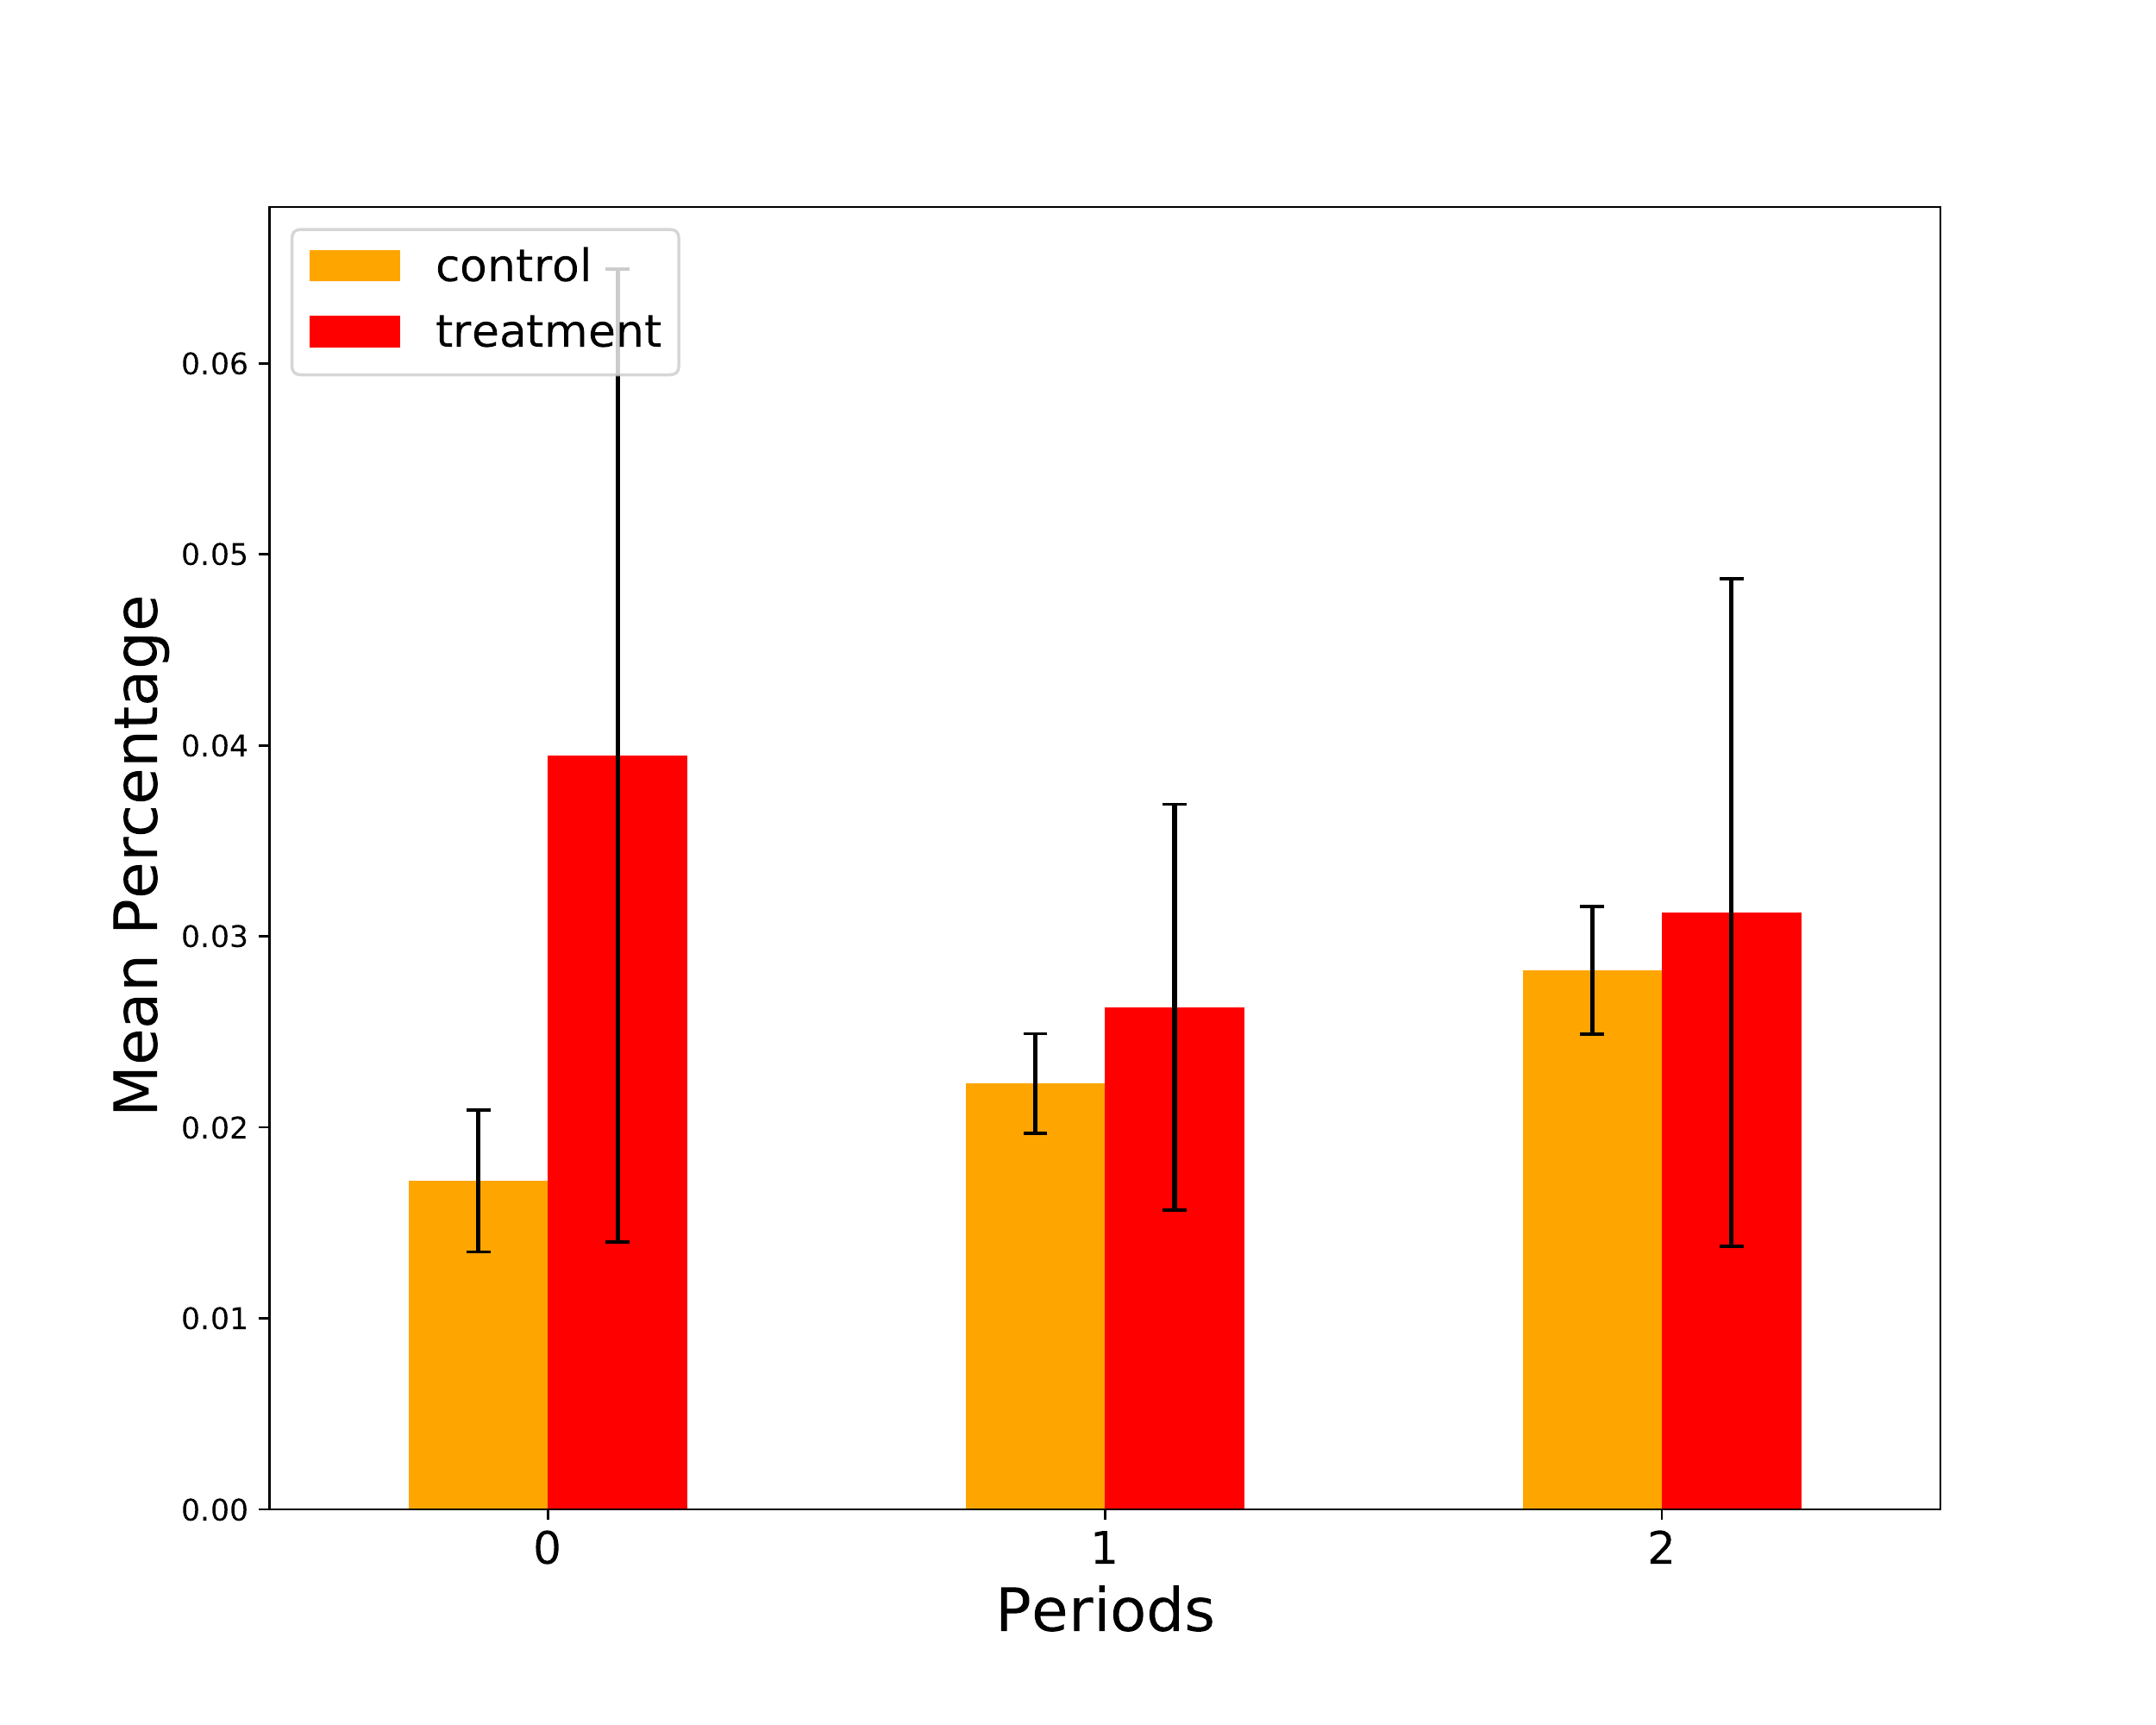}
    \caption{Uncertainty-Economics}
    \label{fig:ds_2a}
  \end{subfigure}
  \hfill
 \begin{subfigure}[h]{0.4\textwidth}
    \includegraphics[width=\textwidth]{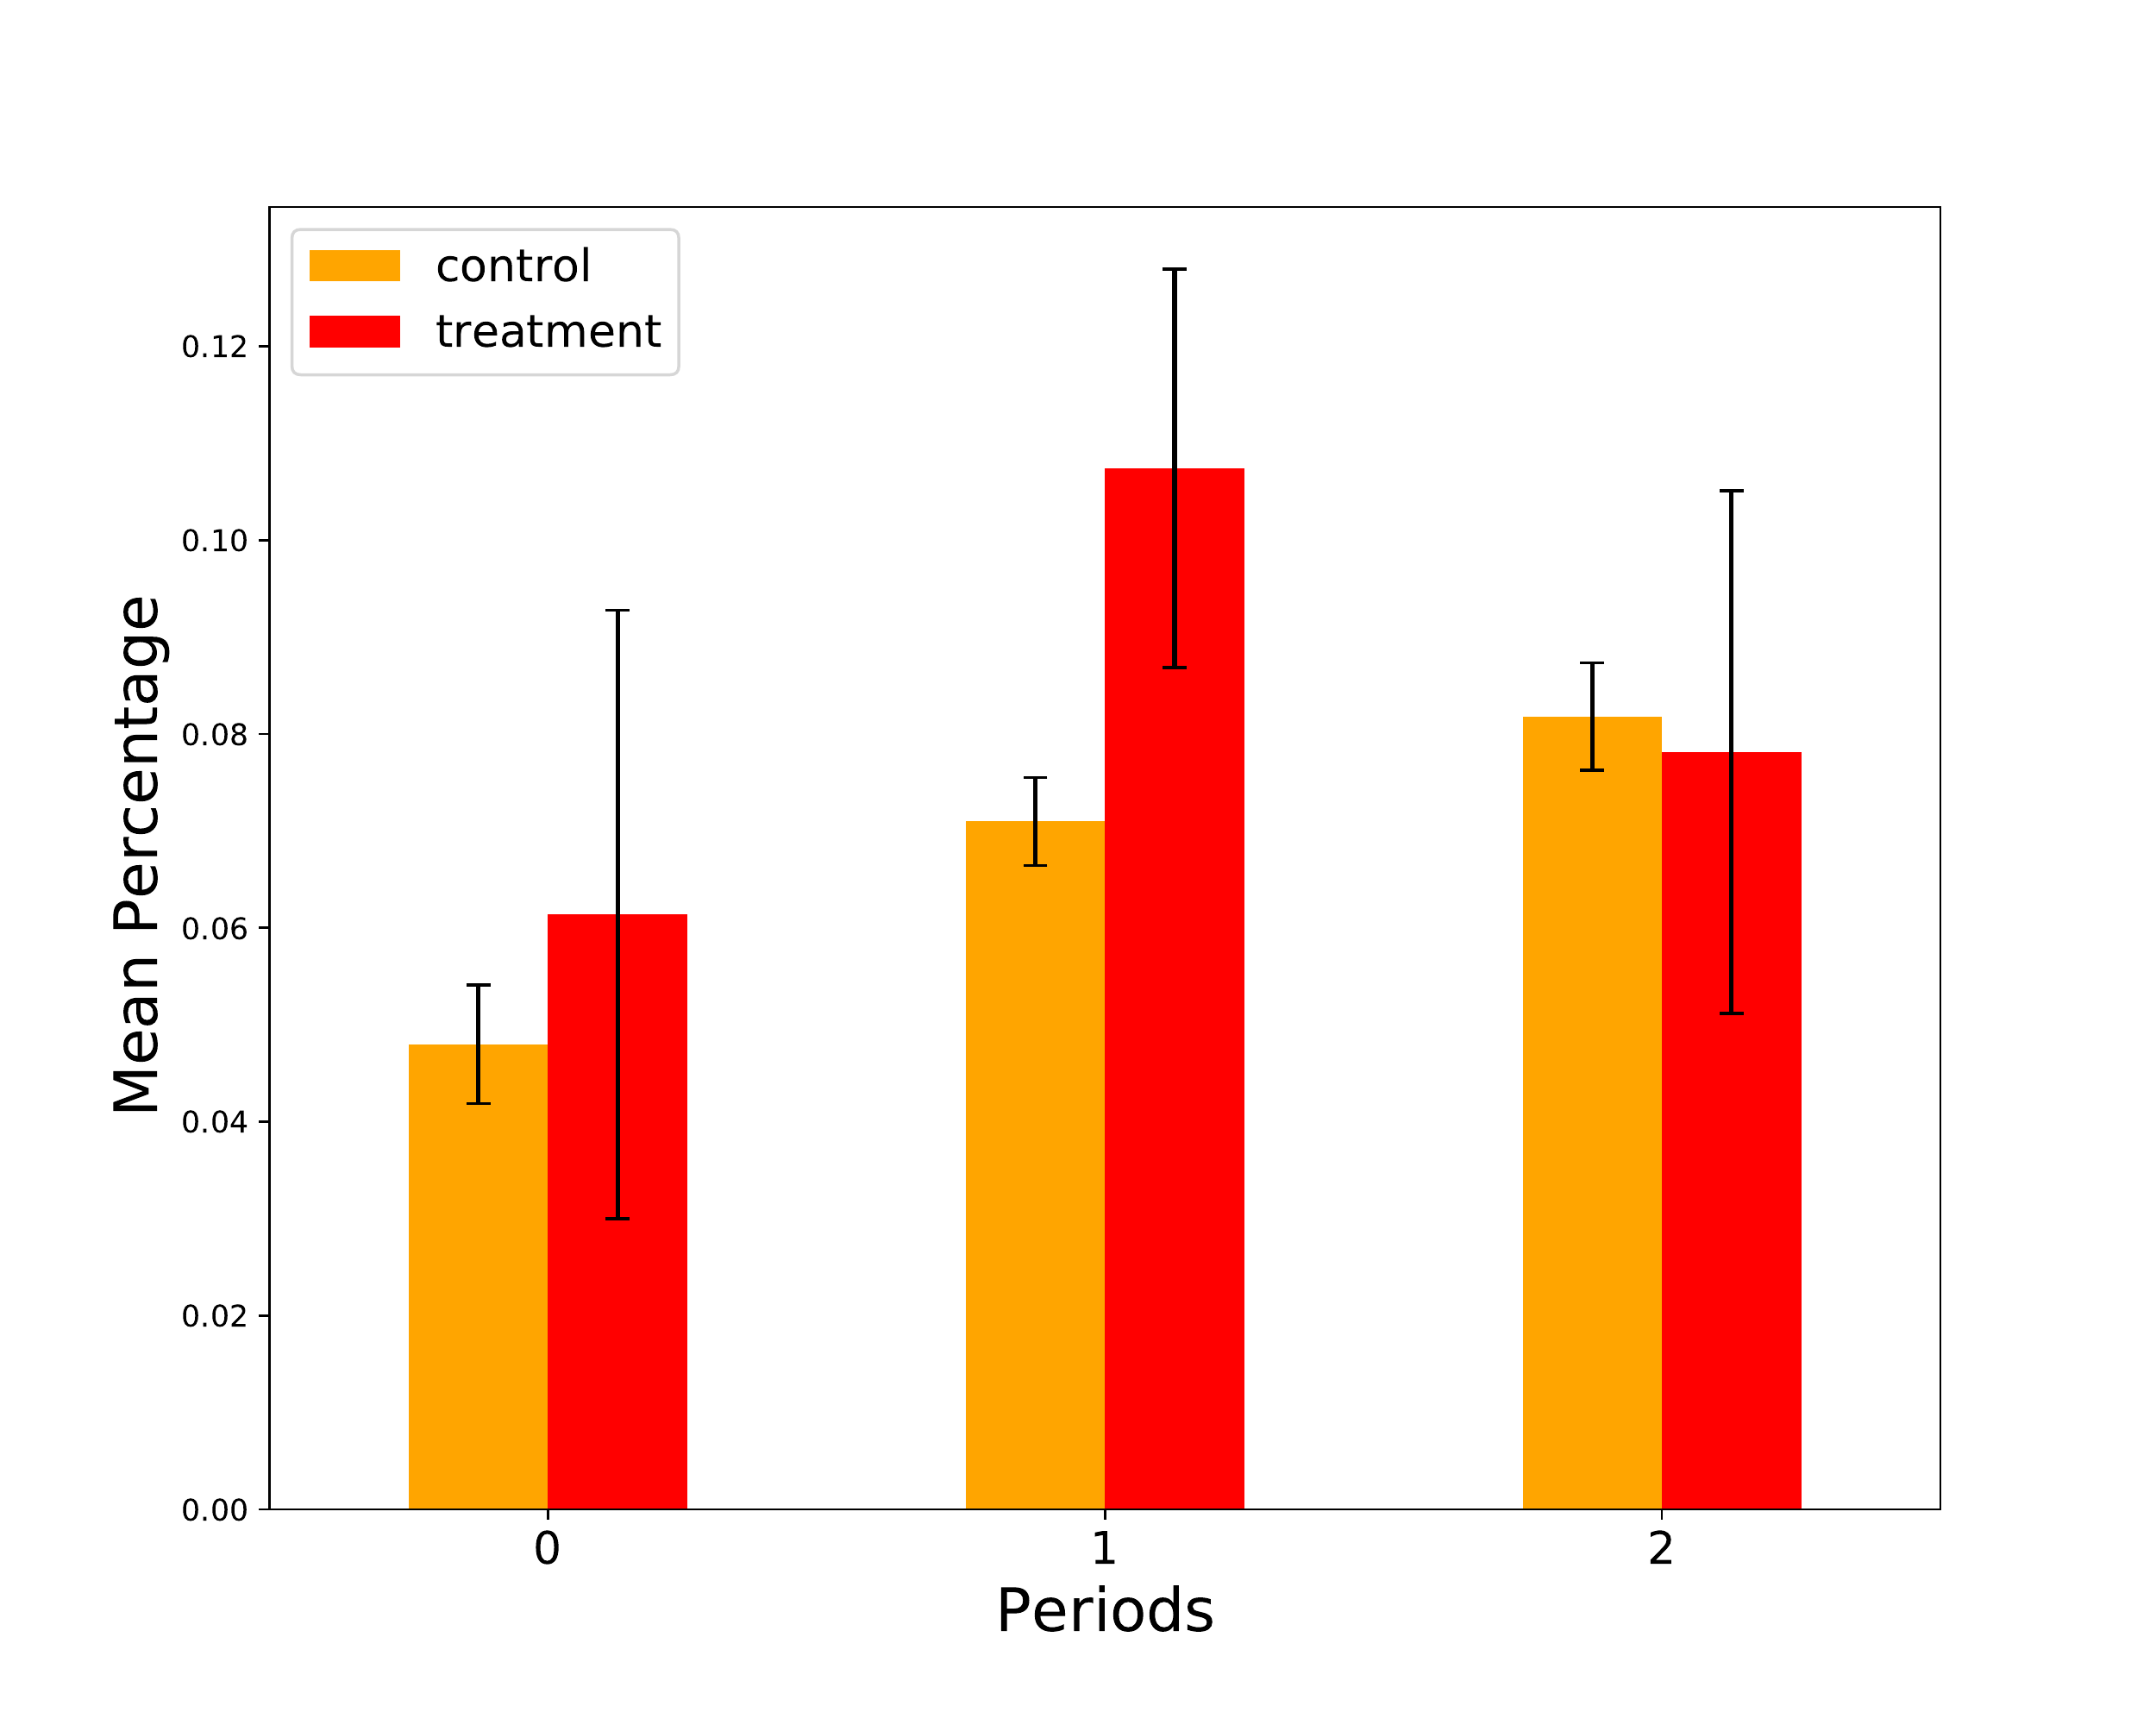}
    \caption{Uncertainty-Health}
    \label{fig:ds_2b}
  \end{subfigure}
  \begin{subfigure}[h]{0.4\textwidth}
    \includegraphics[width=\textwidth]{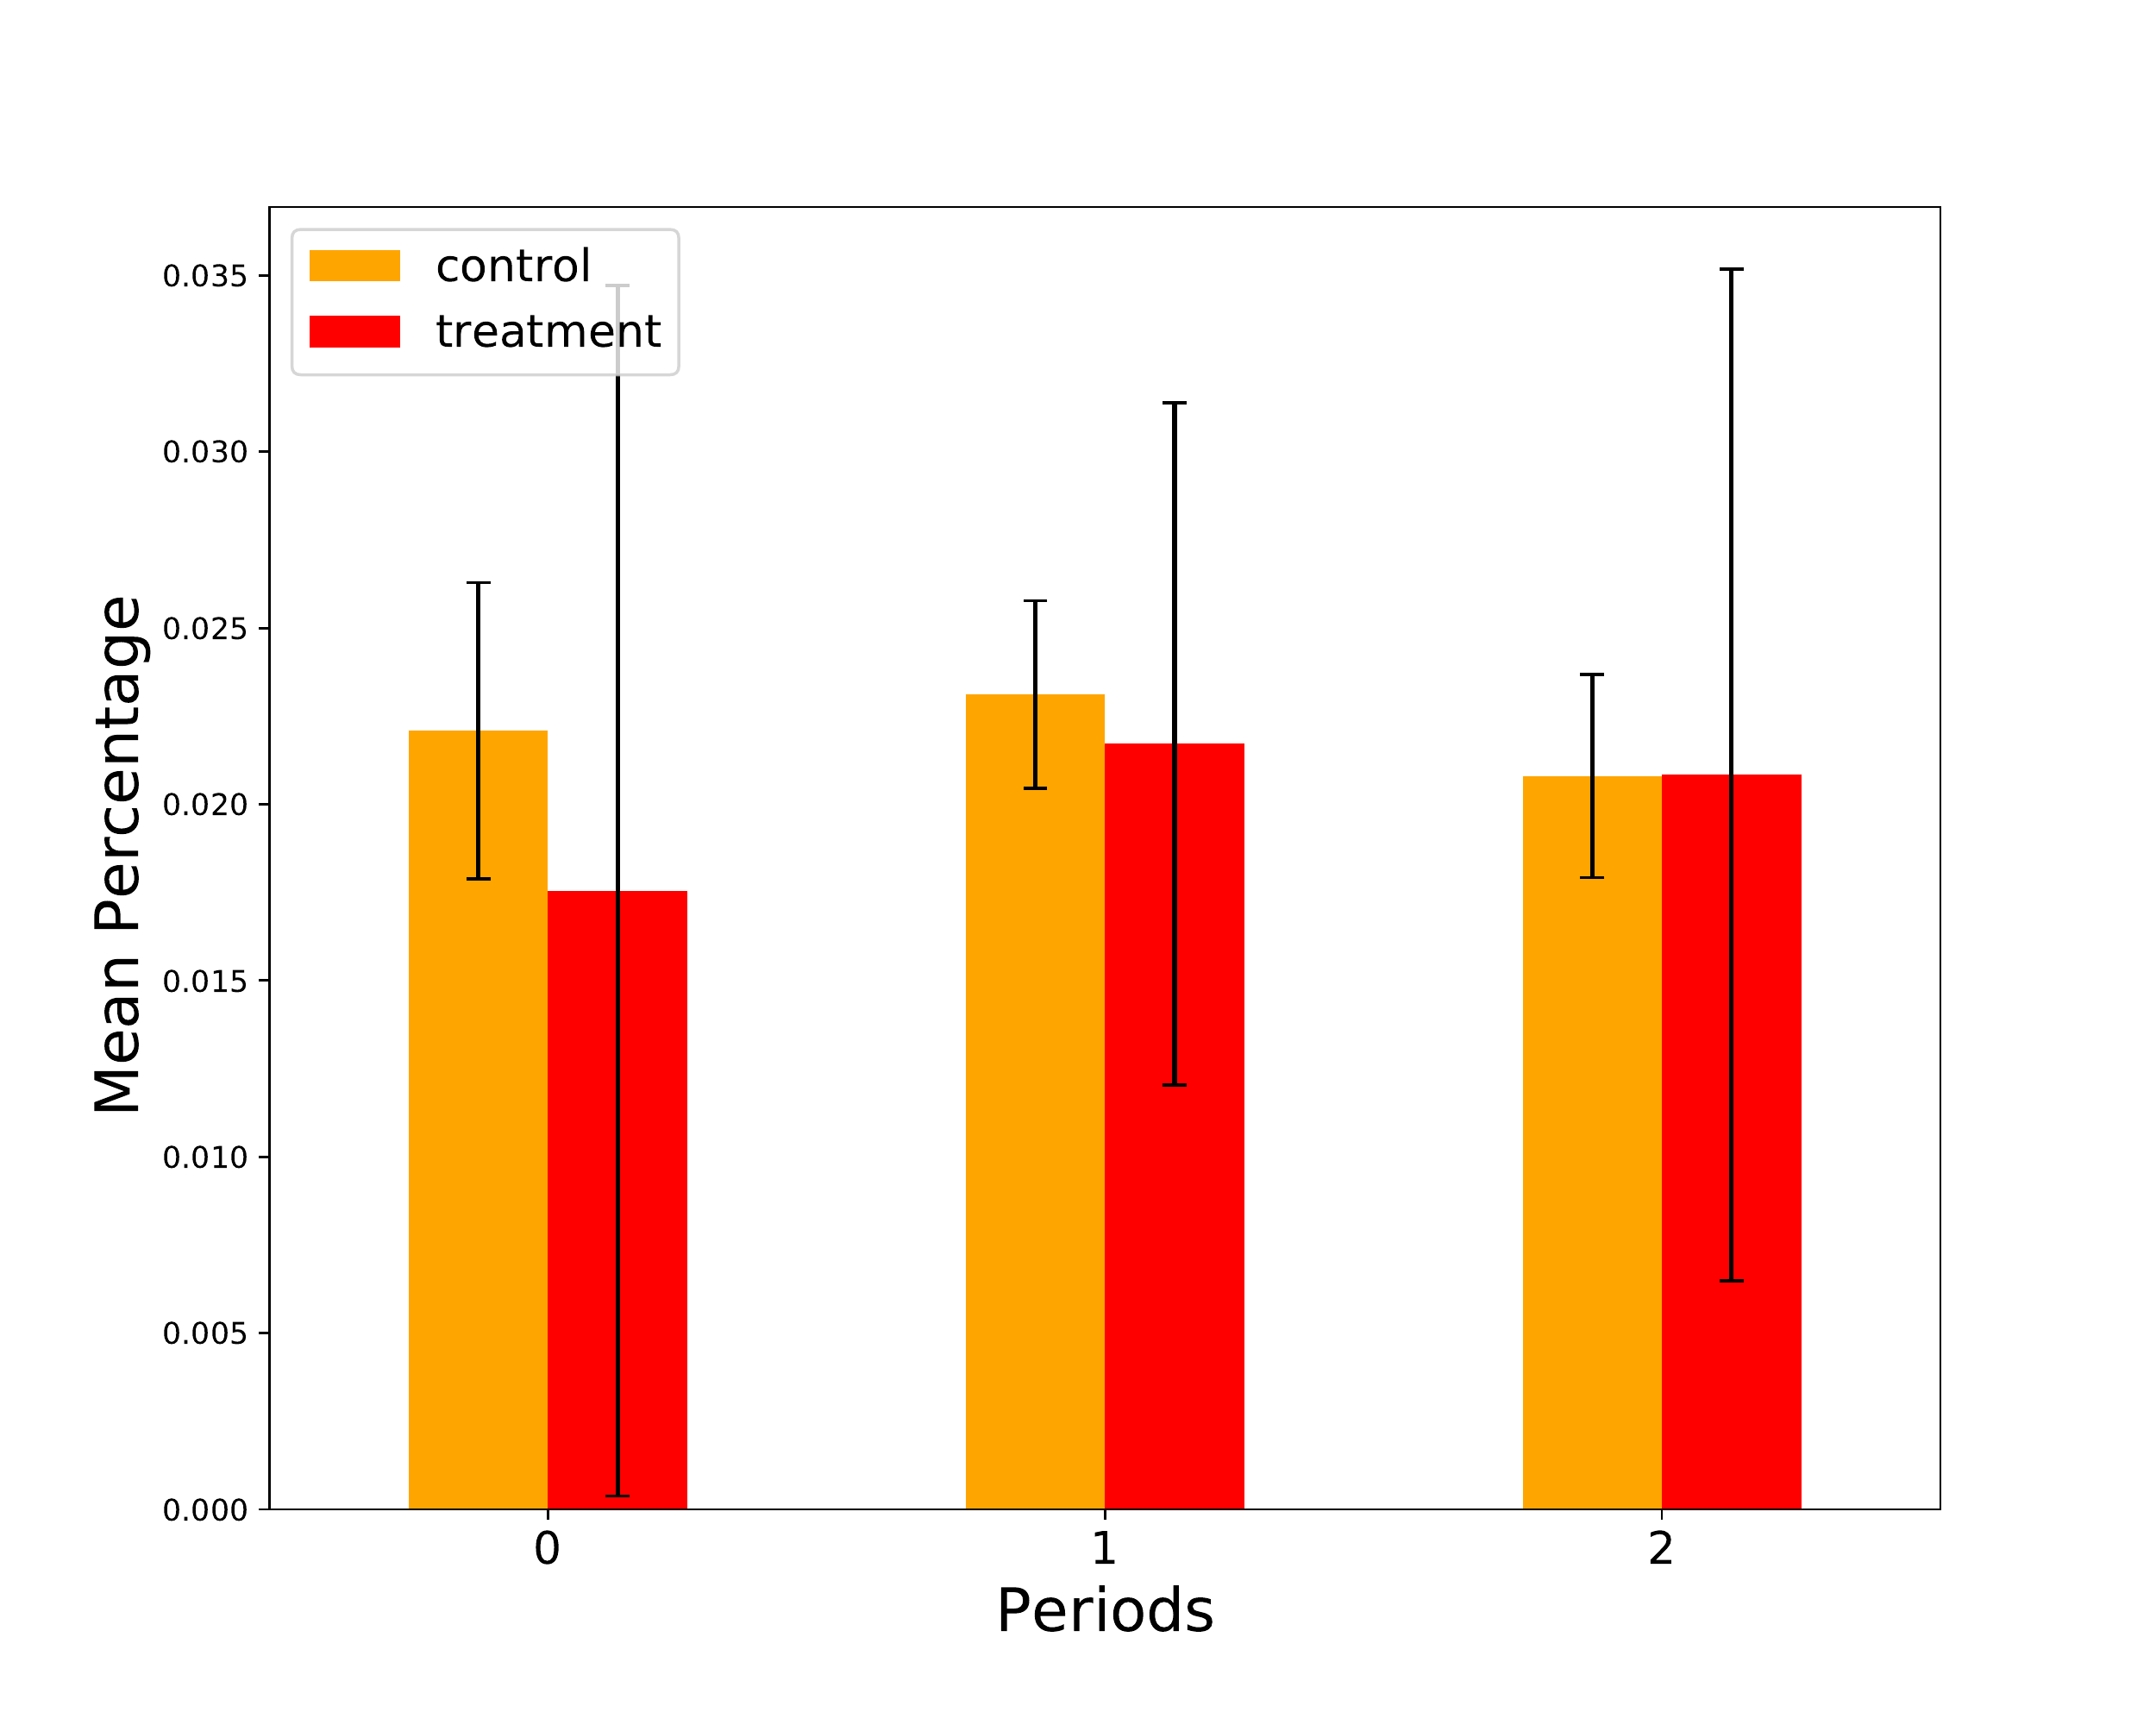}
    \caption{Uncertainty-Politics}
    \label{fig:ds_2c}
  \end{subfigure}
  \hfill
 \begin{subfigure}[h]{0.4\textwidth}
    \includegraphics[width=\textwidth]{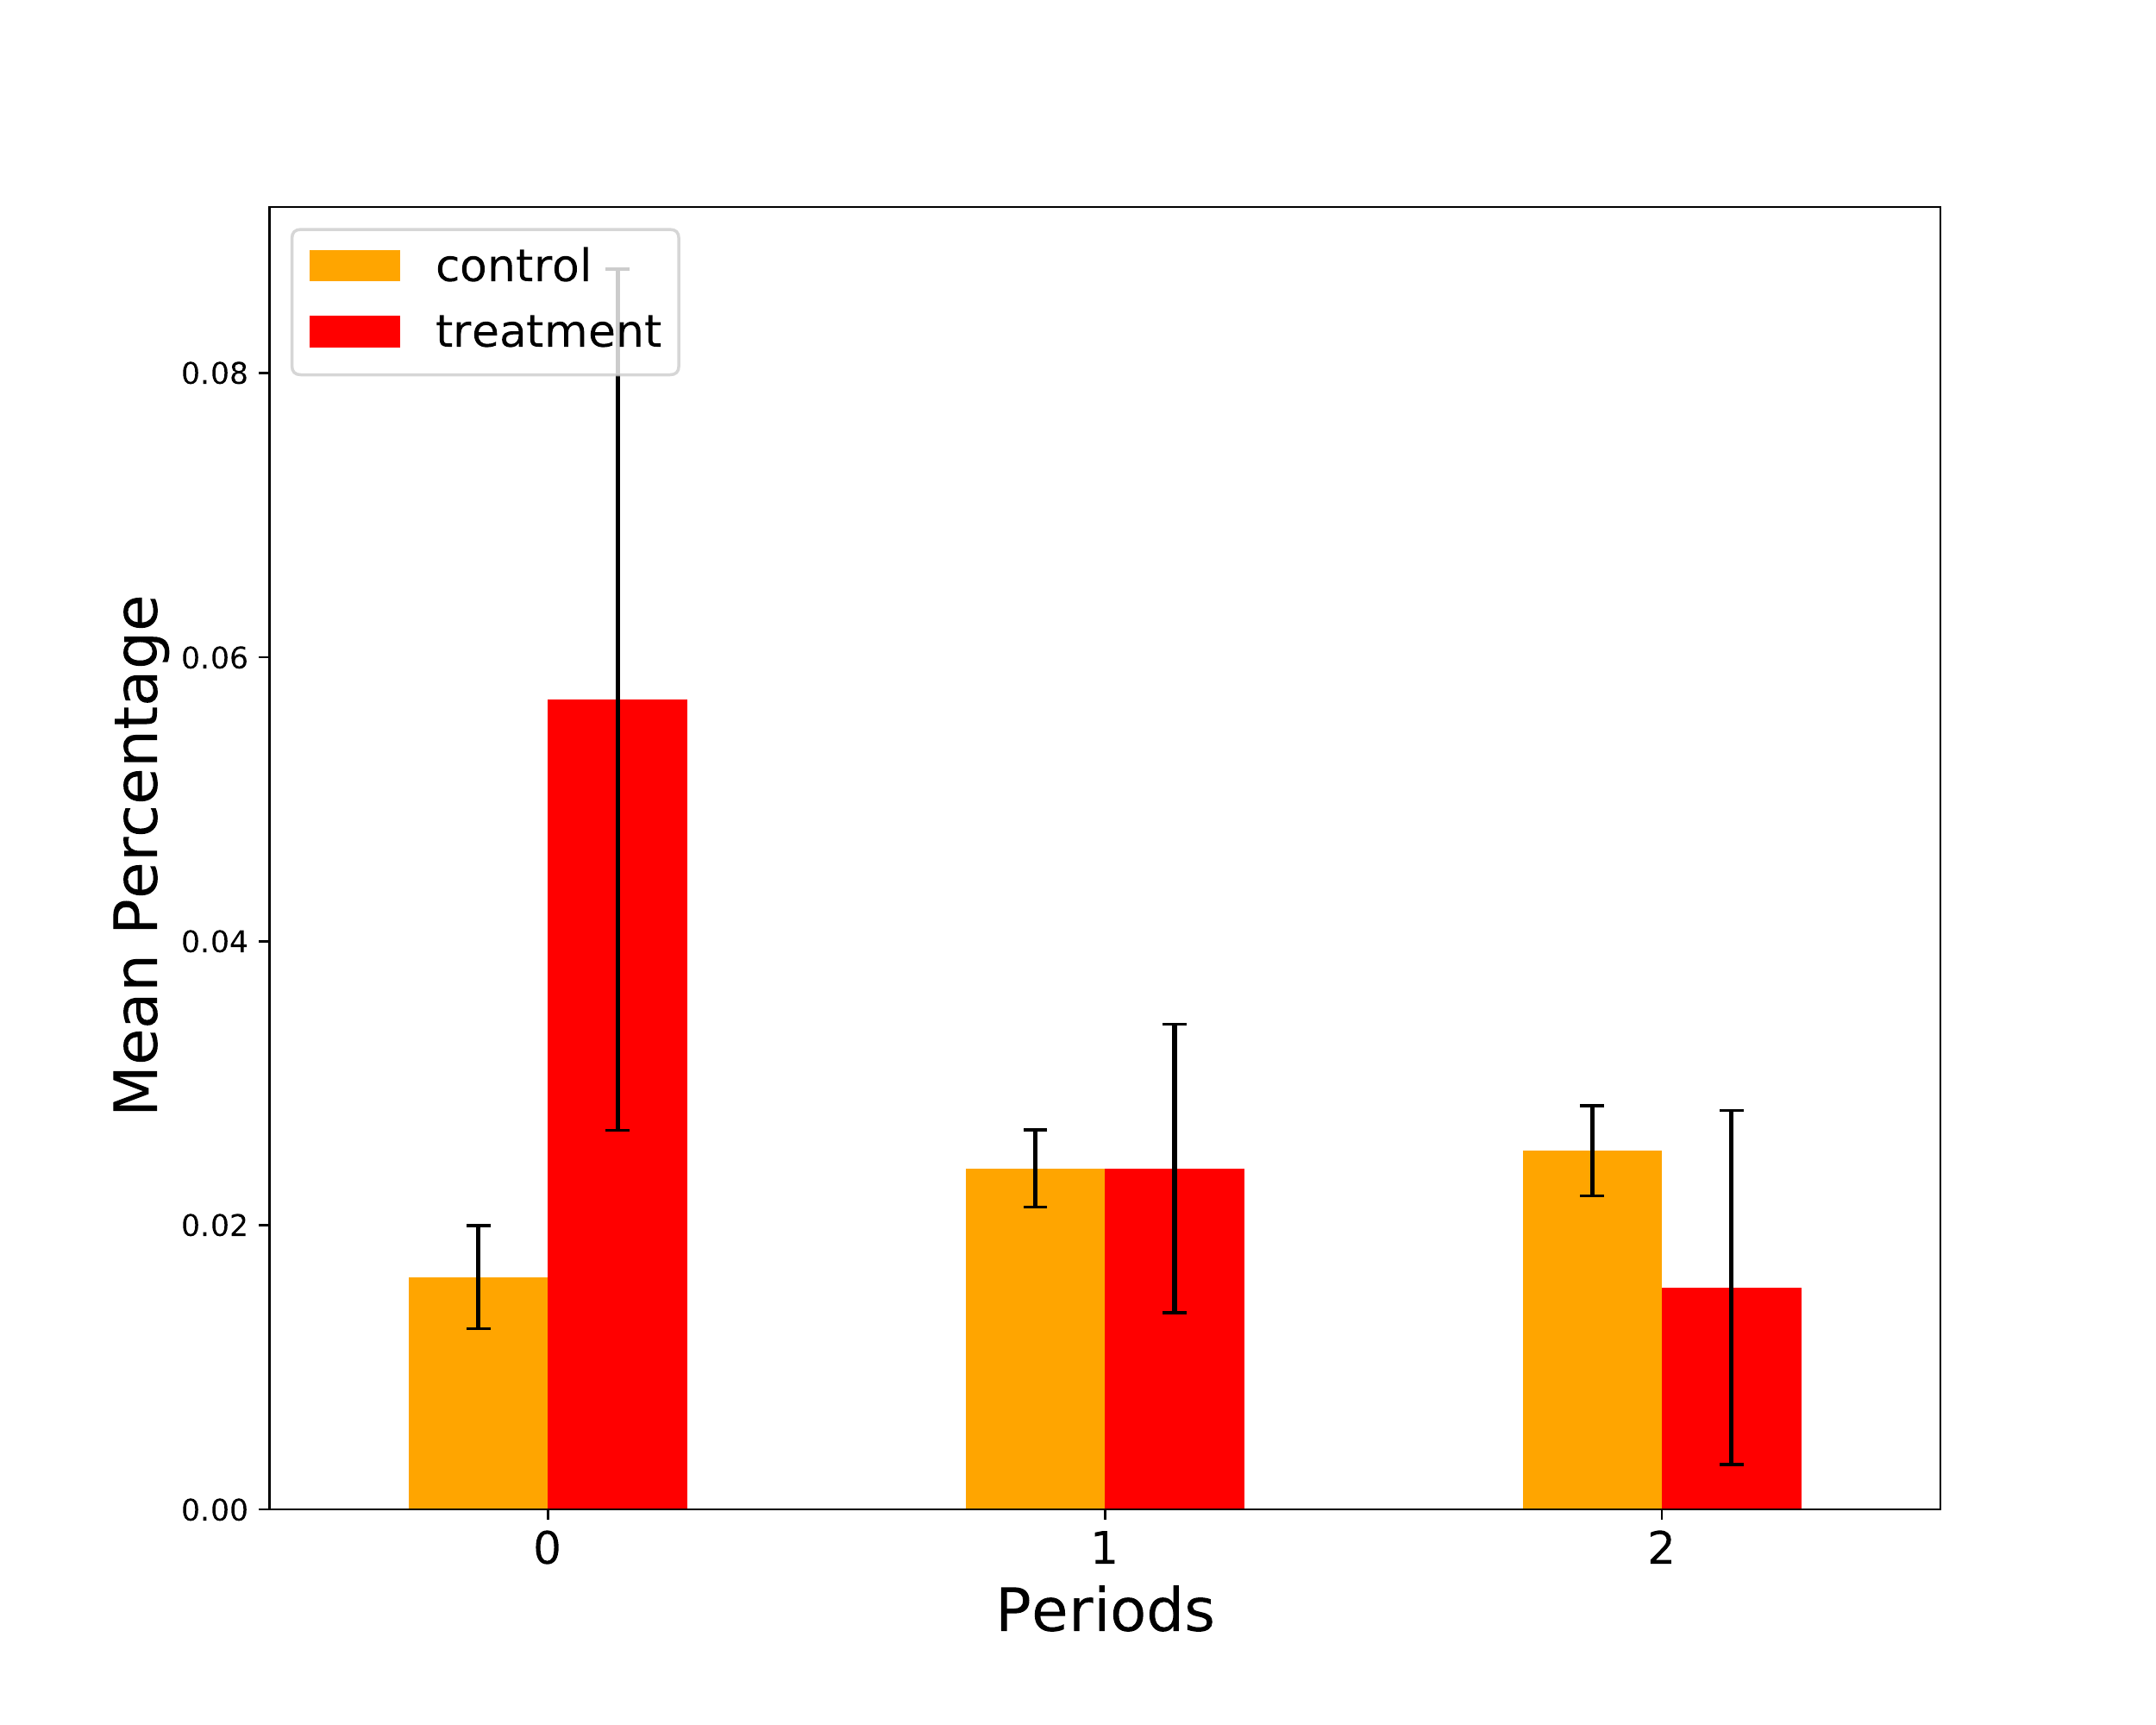}
    \caption{Uncertainty-Lockdown restrictions}
    \label{fig:ds_2d}
  \end{subfigure}
    \begin{subfigure}[h]{0.4\textwidth}
    \includegraphics[width=\textwidth]{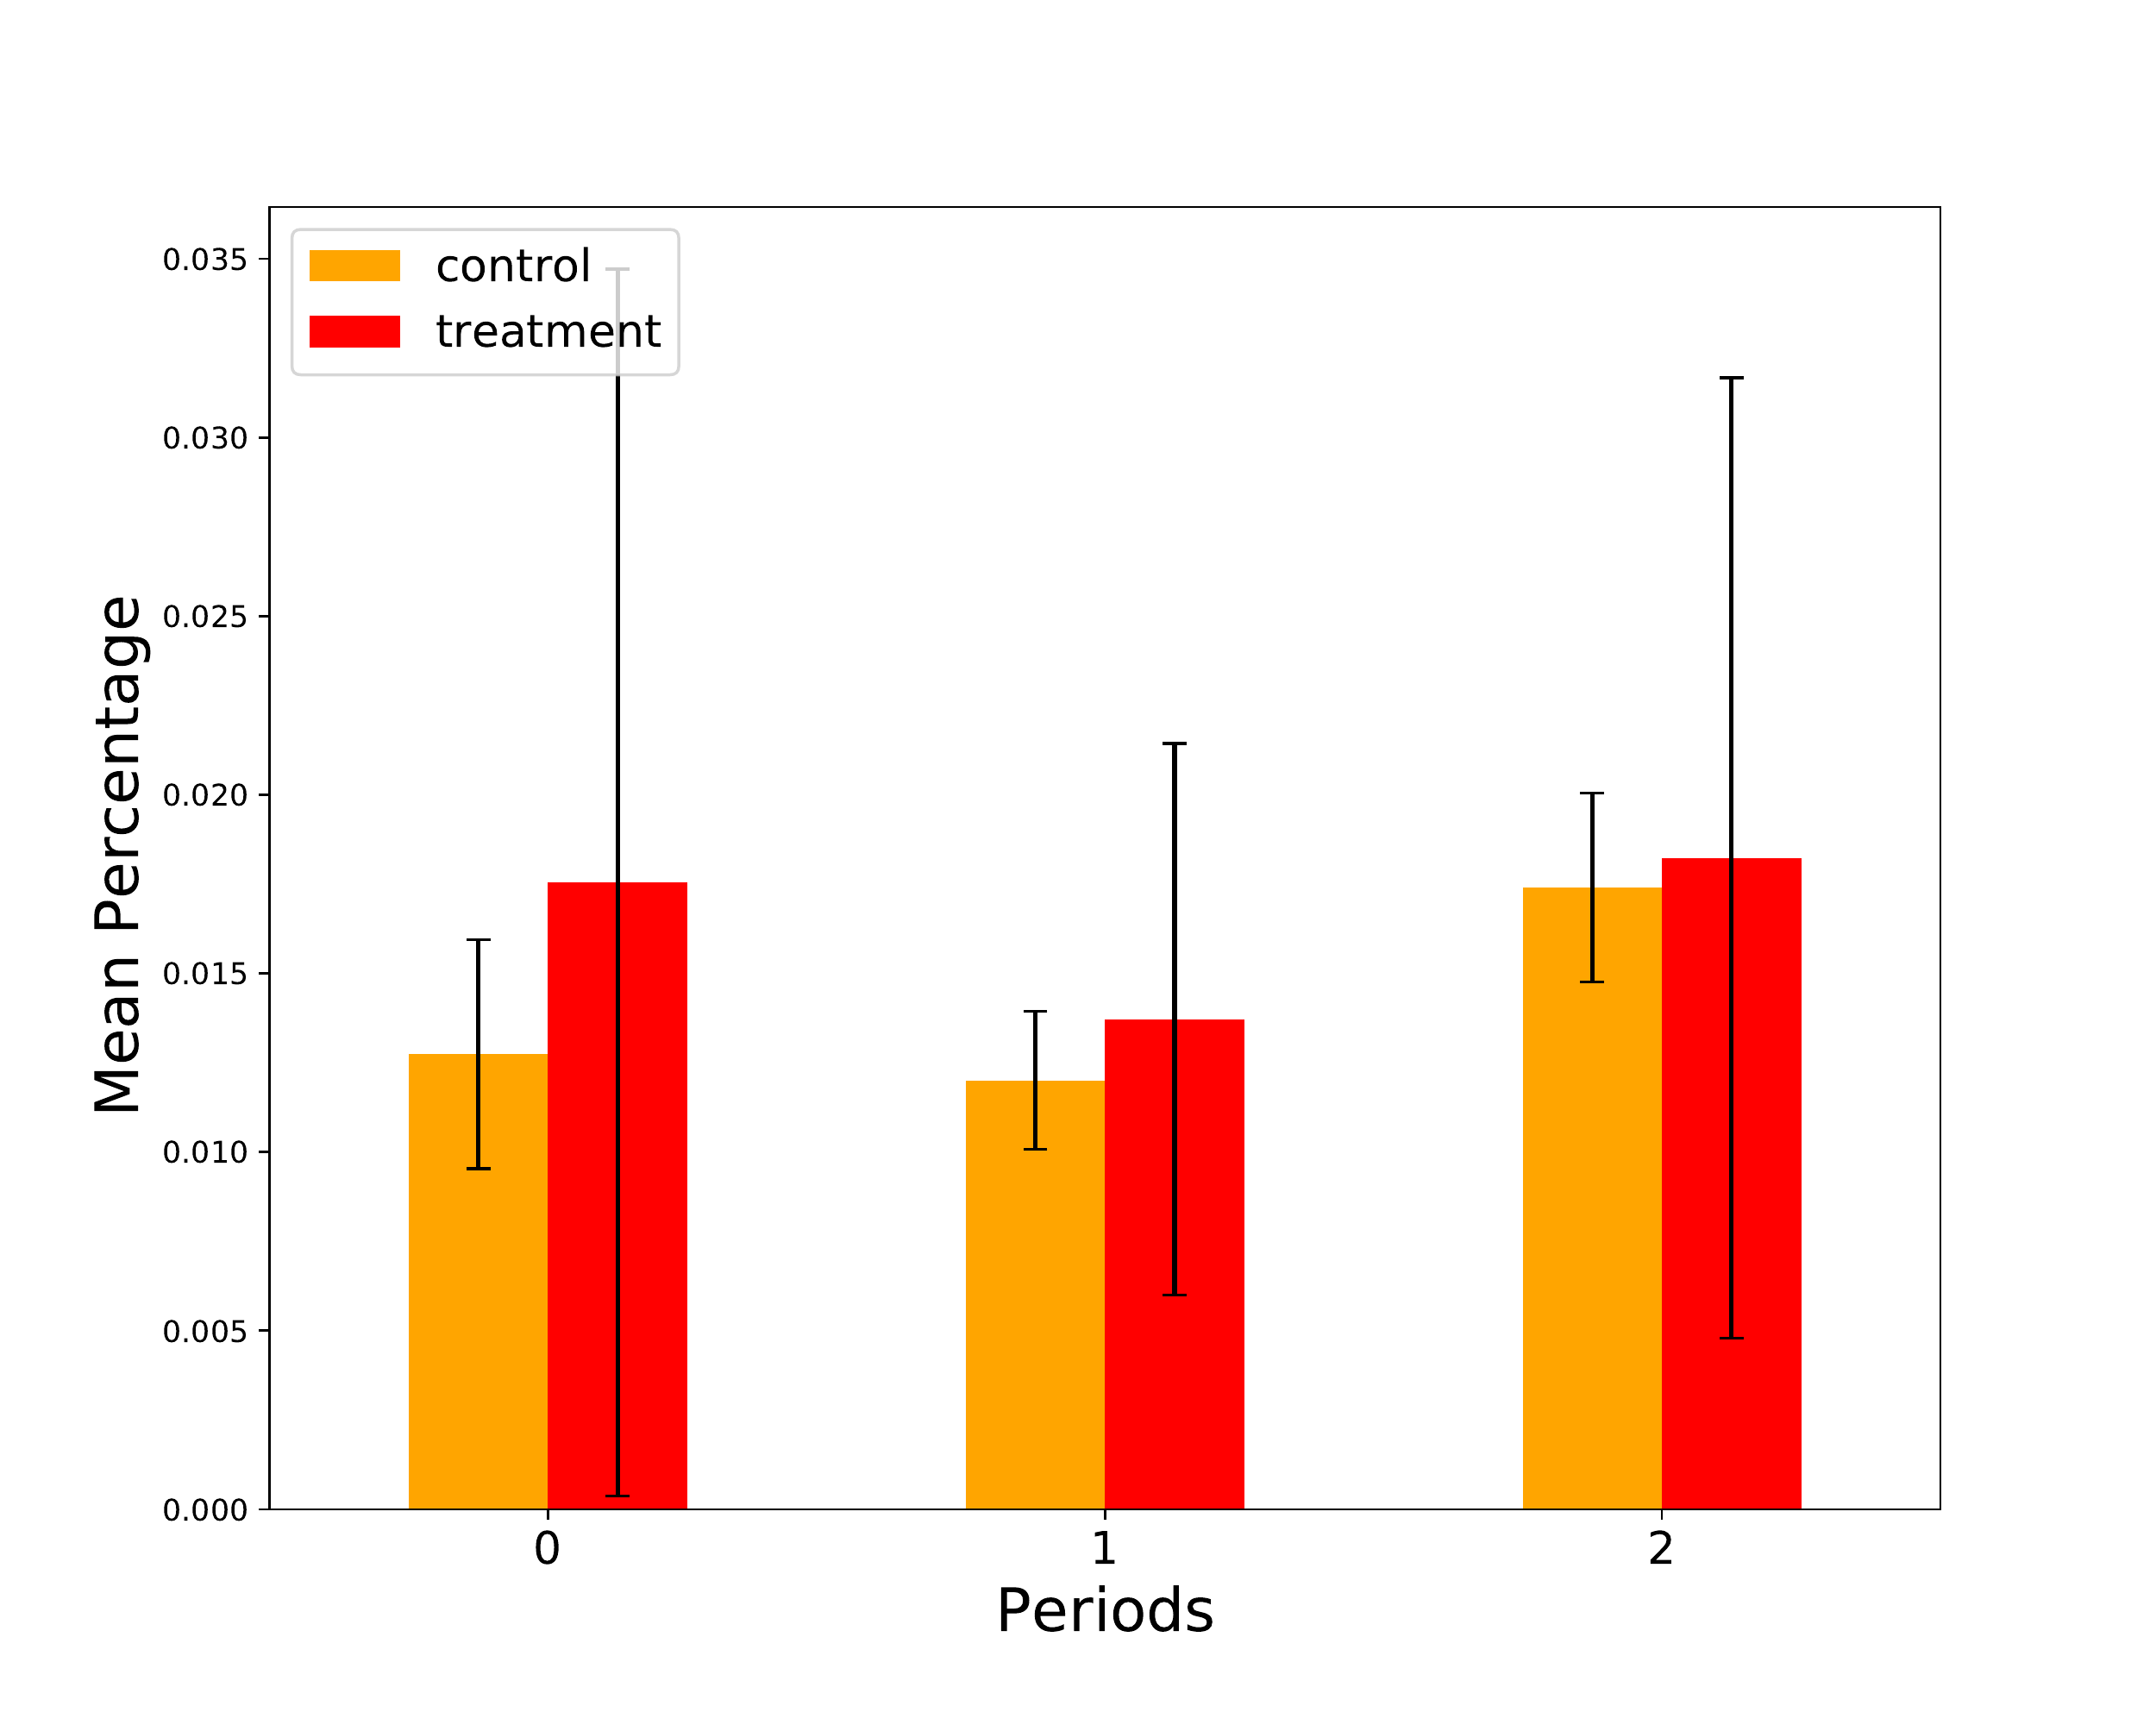}
    \caption{Negative Sentiment-Economics}
    \label{fig:ds_3a}
  \end{subfigure}
  \hfill
 \begin{subfigure}[h]{0.4\textwidth}
    \includegraphics[width=\textwidth]{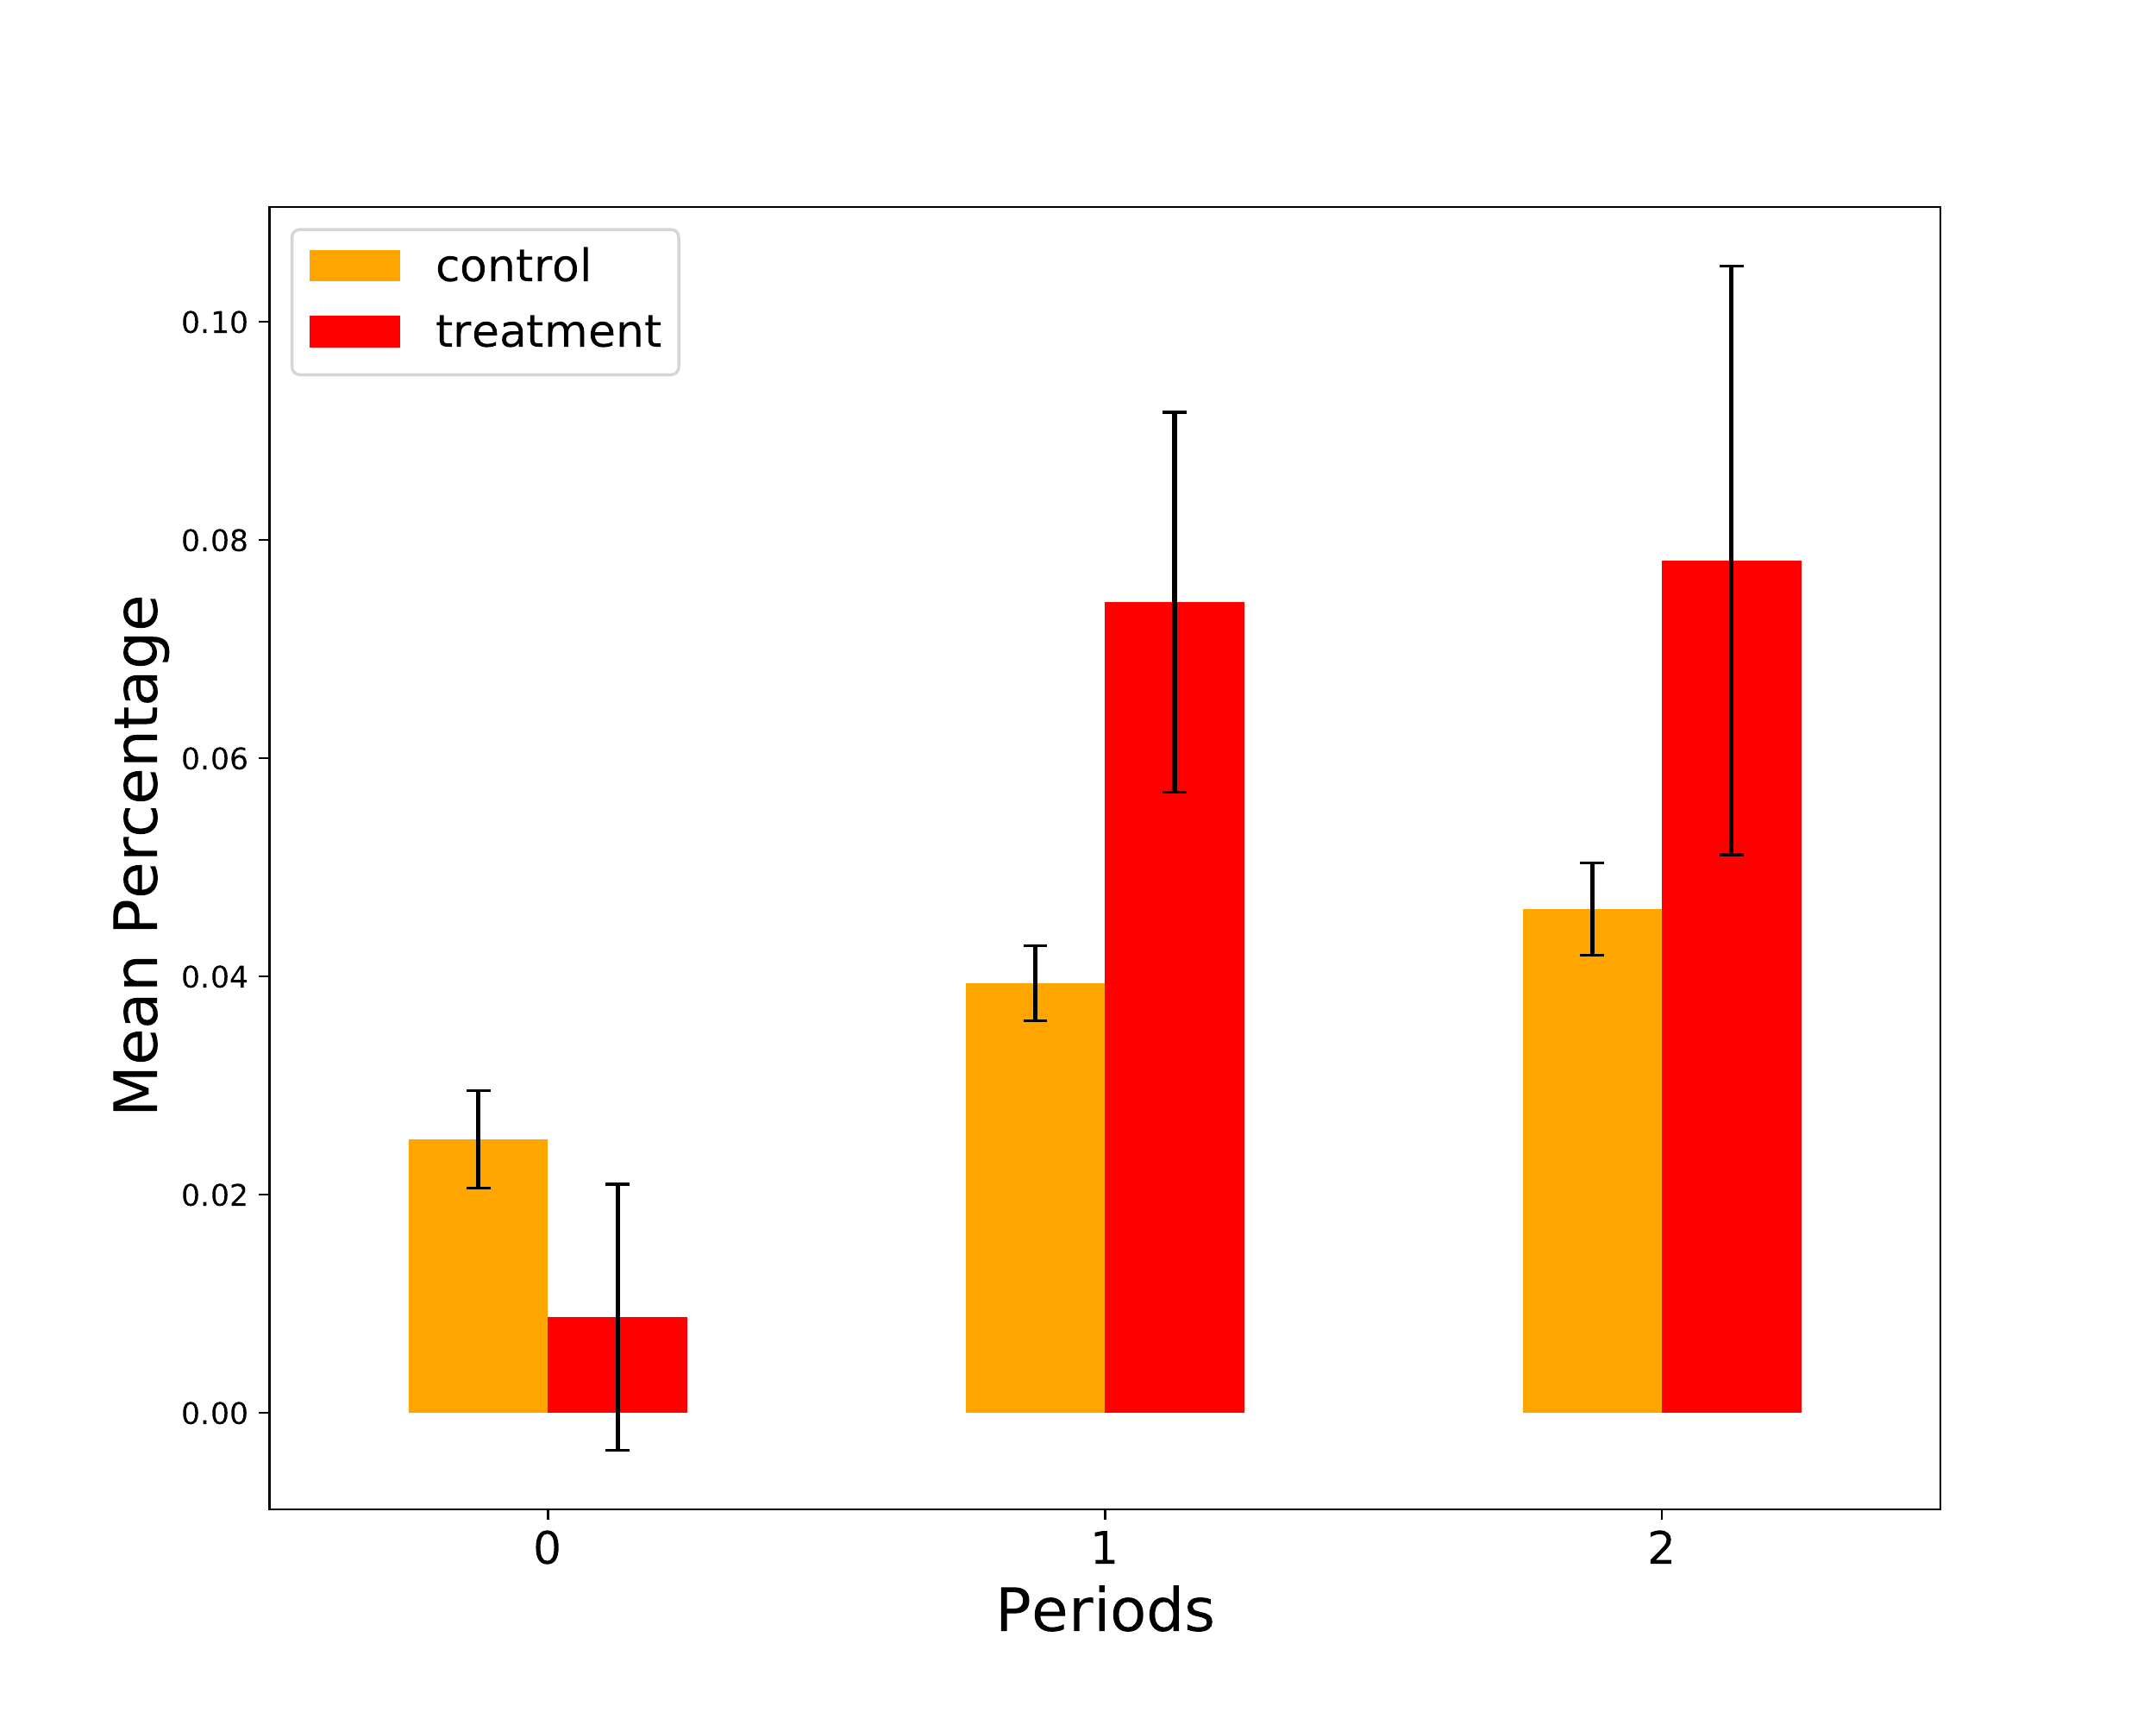}
    \caption{Negative Sentiment-Health}
    \label{fig:ds_3b}
  \end{subfigure}
  \begin{subfigure}[h]{0.4\textwidth}
    \includegraphics[width=\textwidth]{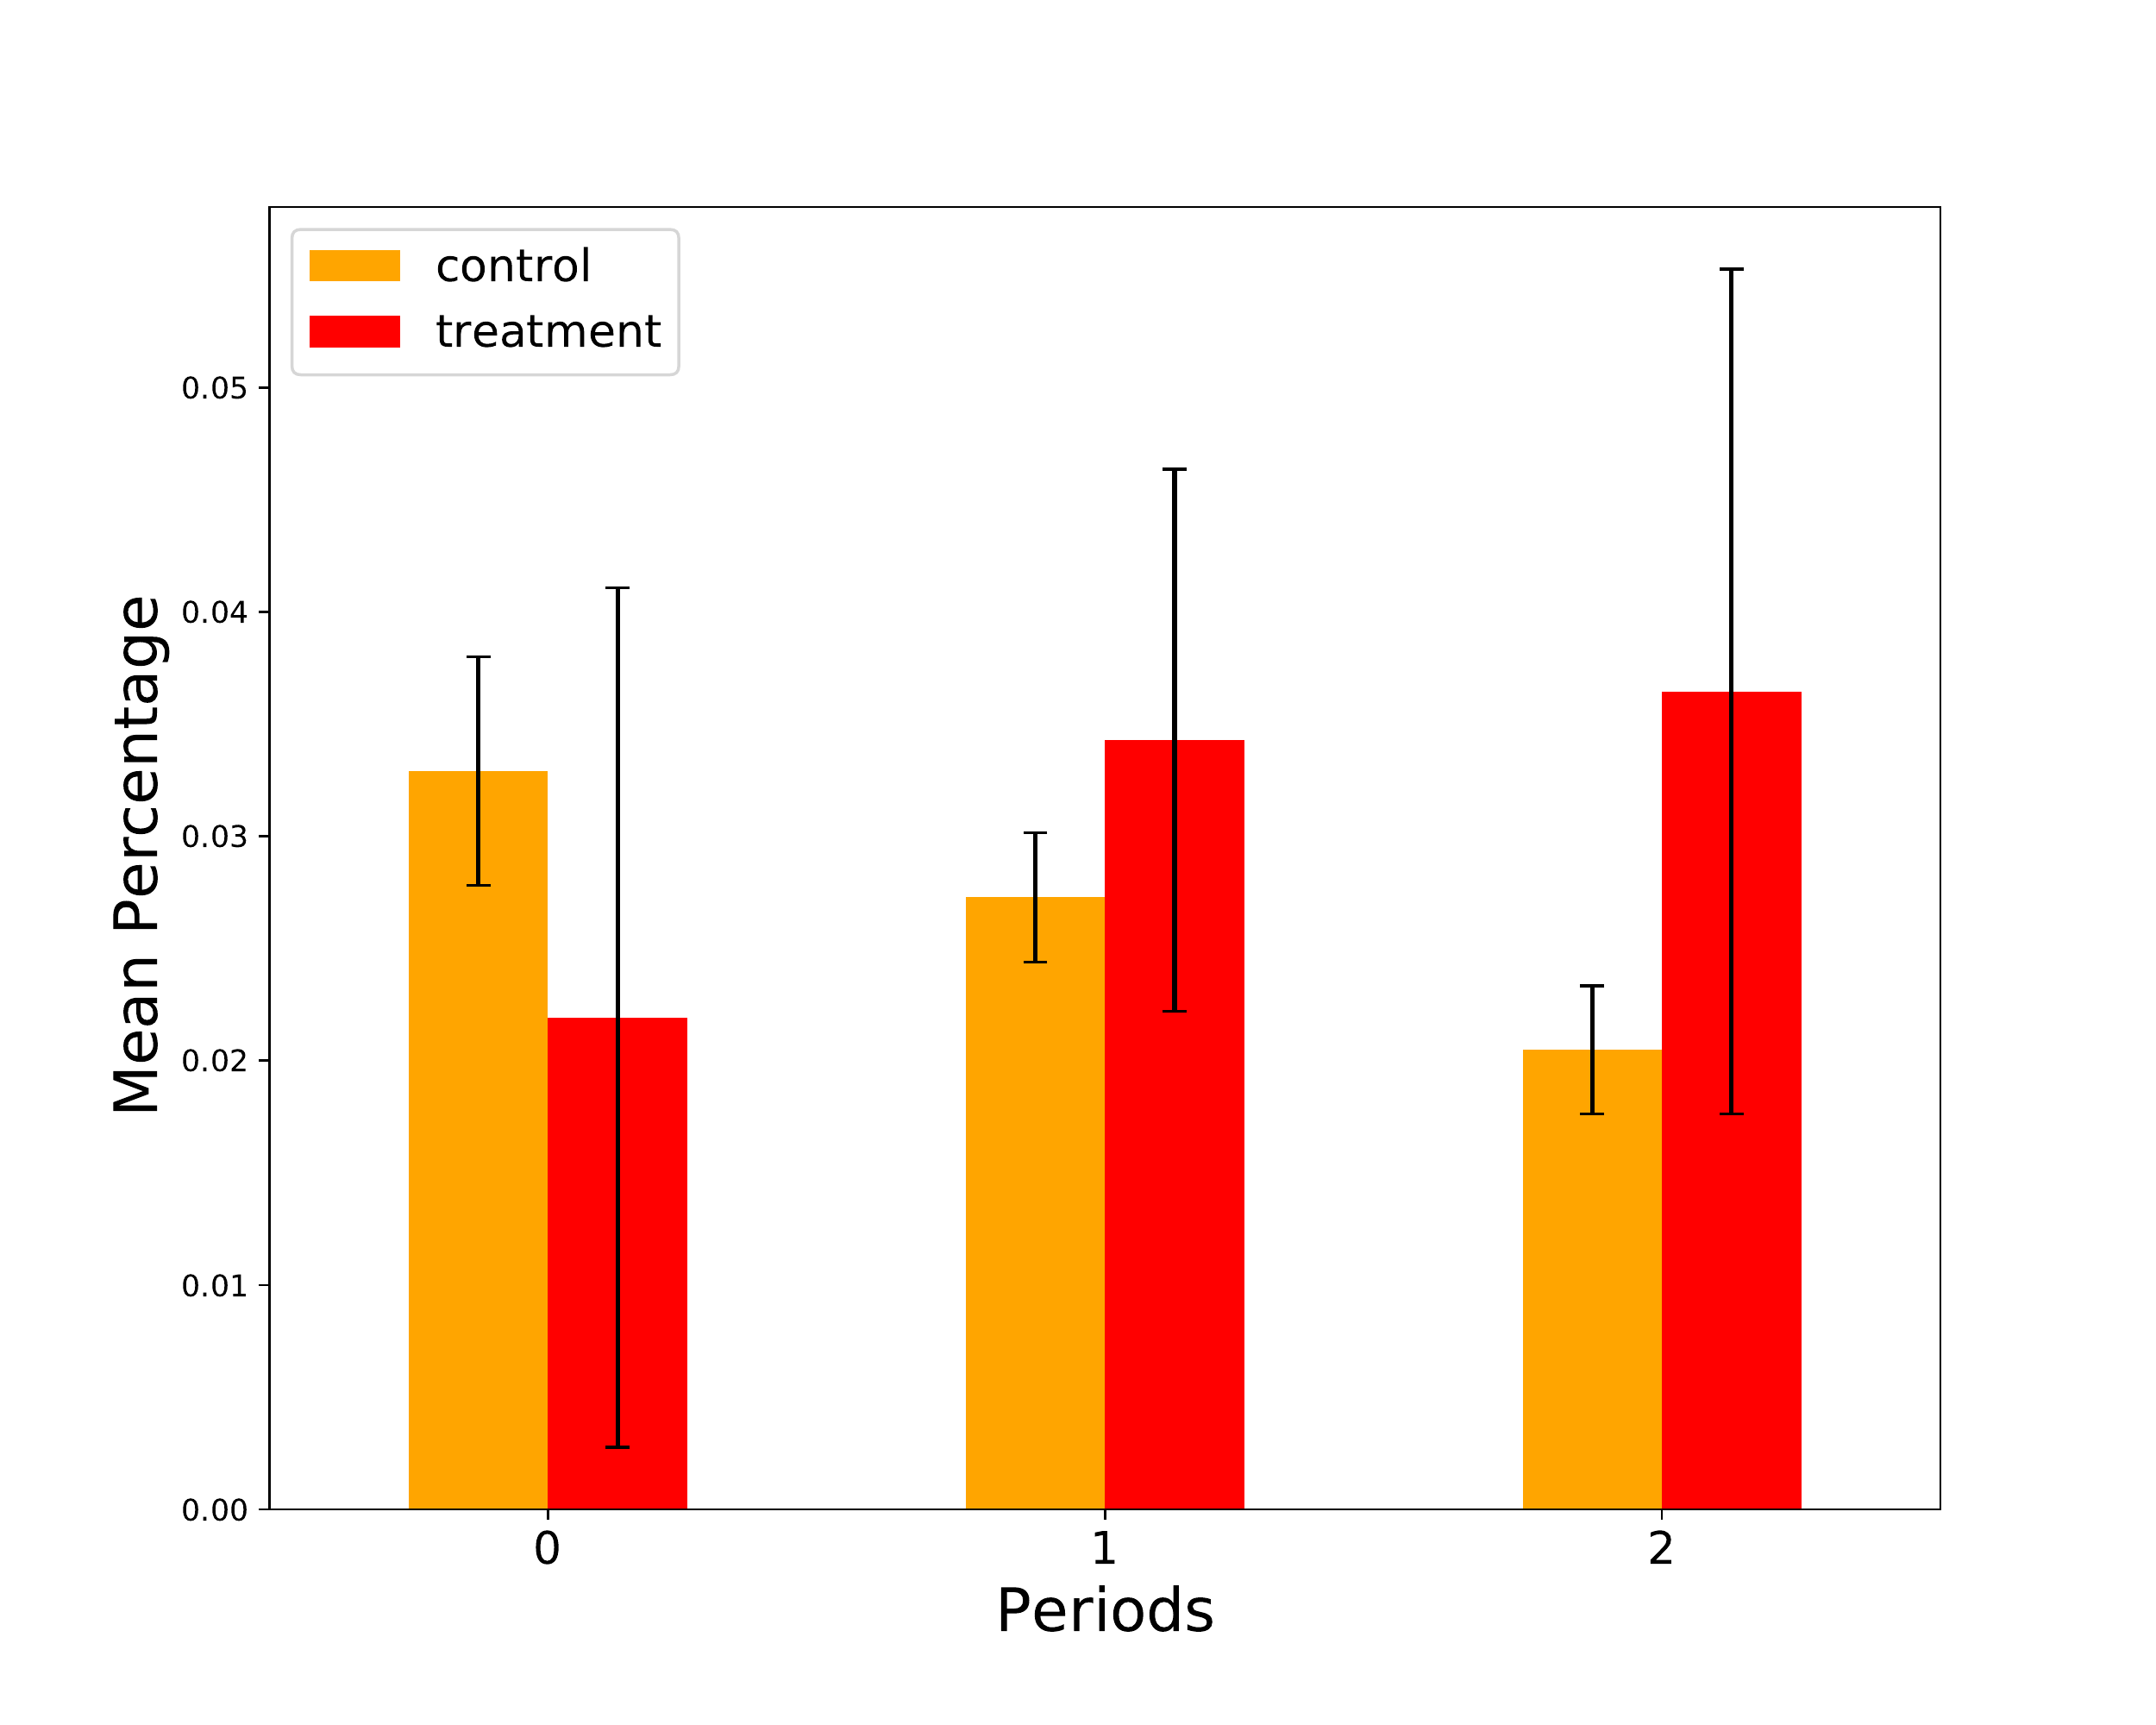}
    \caption{Negative Sentiment-Politics}
    \label{fig:ds_3c}
  \end{subfigure}
  \hfill
 \begin{subfigure}[h]{0.4\textwidth}
    \includegraphics[width=\textwidth]{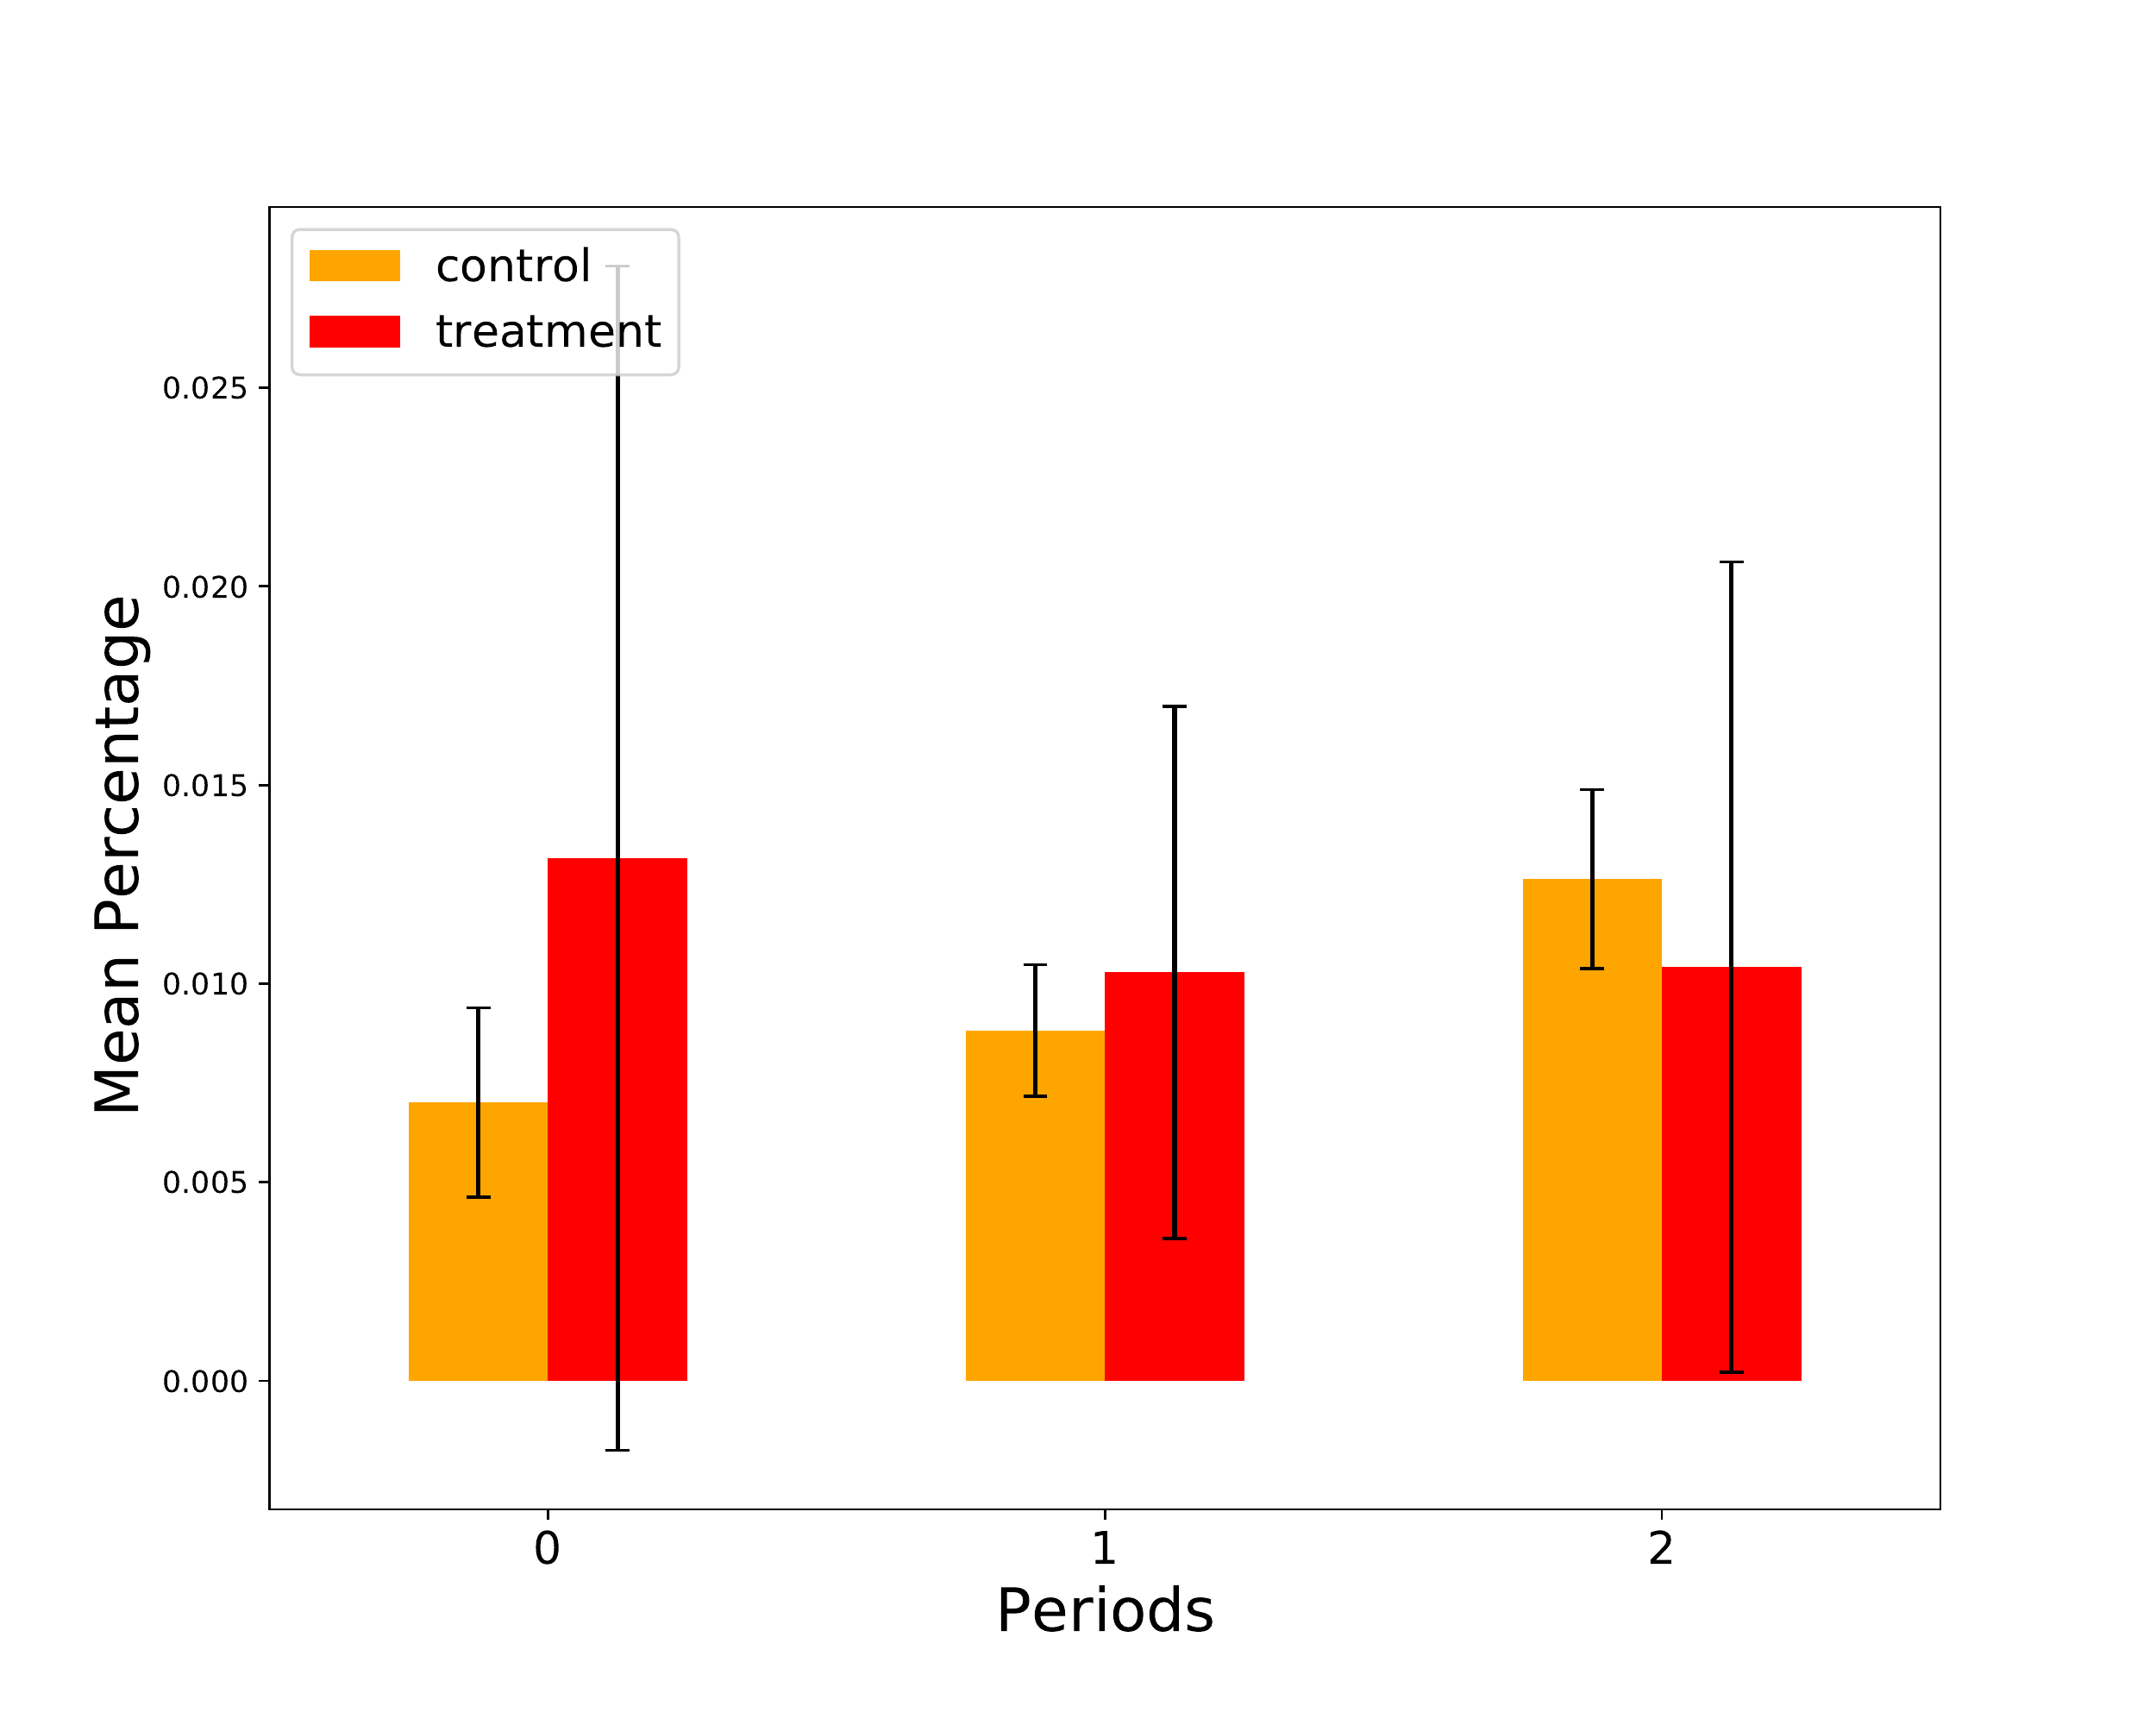}
    \caption{Negative Sentiment-Lockdown restrictions}
    \label{fig:ds_3d}
  \end{subfigure}
  \caption{Share of tweets expressing \emph{Uncertainty} and \emph{Negative Sentiment} grouped by \emph{Topics} categories for \emph{control} and \emph{treated} cities.}
  \label{fig:ds_2}
\end{figure}

\end{document}
