# Supplementary material for: Breaking Down the Lockdown: The Causal Effects of Stay-At-Home Mandates on Uncertainty and Sentiments During the COVID-19 Pandemic
Source: arXiv:2212.01705 source file (2023-06-01)
Supplement: Supplementary file 4 [file grouped_FEs.tex]

\documentclass[../main.tex]{subfiles}
\begin{document}
We modify the DID model by including \emph{municipality} level fixed effects, in order to tackle any possible source of omitted variable bias coming from city-level heterogeneity. 

%We keep the standard errors clustered at the city-level and re-estimate the models.
We find that the effect of the lockdown is still significant and matches the previous results found for health and political uncertainty and negative sentiments related to health and politics. 

%On the other hand, we lose any effect of the lockdown on health-related uncertainty. This indicates that the differential we found previously on health-related uncertainty between treated and control groups can actually be explained by the fixed heterogeneity at the city-level. 

\begin{table}[H]\centering
\def\sym#1{\ifmmode^{#1}\else\(^{#1}\)\fi}
\caption{DID estimates for \emph{Uncertainty} and \emph{Negative Sentiment}, municipality fixed effects (omitted).}
\begin{adjustbox}{max width=\textwidth}
\begin{tabular}{lrrrrrrrrrr}
\toprule
&\multicolumn{5}{c}{Uncertainty}&\multicolumn{5}{c}{Negative Sentiment}\\
\toprule
                    &\multicolumn{1}{c}{(1)}&\multicolumn{1}{c}{(2)}&\multicolumn{1}{c}{(3)}&\multicolumn{1}{c}{(4)}&\multicolumn{1}{c}{(5)}&\multicolumn{1}{c}{(6)}&\multicolumn{1}{c}{(7)}&\multicolumn{1}{c}{(8)}&\multicolumn{1}{c}{(9)}&\multicolumn{1}{c}{(10)}\\
                    &\multicolumn{1}{c}{All}&\multicolumn{1}{c}{Economics}&\multicolumn{1}{c}{Health}&\multicolumn{1}{c}{Politics}&\multicolumn{1}{c}{Policy}&\multicolumn{1}{c}{All}&\multicolumn{1}{c}{Economics}&\multicolumn{1}{c}{Health}&\multicolumn{1}{c}{Politics}&\multicolumn{1}{c}{Policy}\\
\midrule
post=1              &      0.0571\sym{***}&     0.00902\sym{***}&      0.0614\sym{***}&   -0.000821         &      0.0205\sym{***}&     -0.0280         &    -0.00430         &      0.0356\sym{***}&    -0.00776         &     0.00641\sym{**} \\
                    &      (5.76)         &      (4.57)         &      (7.04)         &     (-0.21)         &     (10.16)         &     (-0.98)         &     (-1.86)         &      (5.23)         &     (-1.28)         &      (2.85)         \\
\addlinespace
post=2              &      0.0663\sym{***}&      0.0152\sym{***}&      0.0693\sym{***}&    -0.00128         &      0.0200\sym{***}&     -0.0515\sym{*}  &     0.00107         &      0.0400\sym{***}&     -0.0168\sym{***}&     0.00812\sym{*}  \\
                    &      (5.50)         &      (5.23)         &      (8.97)         &     (-0.36)         &      (6.63)         &     (-2.08)         &      (0.31)         &      (6.26)         &     (-3.40)         &      (2.46)         \\
\addlinespace
red zone=1 $\times$ post=1&      0.0315         &     -0.0135\sym{***}&      0.0299\sym{*}  &      0.0164\sym{**} &     0.00809         &    -0.00863         &     -0.0213         &      0.0464\sym{*}  &      0.0480\sym{***}&      0.0155         \\
                    &      (0.31)         &     (-4.25)         &      (1.98)         &      (2.68)         &      (0.54)         &     (-0.26)         &     (-1.82)         &      (2.48)         &      (5.84)         &      (1.06)         \\
\addlinespace
red zone=1 $\times$ post=2&     -0.0160         &     -0.0114         &    -0.00284         &     0.00524         &     -0.0101\sym{*}  &      0.0156         &     -0.0109         &      0.0537\sym{*}  &      0.0702\sym{***}&     0.00321         \\
                    &     (-0.33)         &     (-1.14)         &     (-0.11)         &      (1.36)         &     (-2.48)         &      (0.38)         &     (-0.62)         &      (2.15)         &      (6.04)         &      (0.87)         \\
\addlinespace
Constant            &       0.221\sym{***}&      0.0568\sym{***}&      0.0126         &    0.000988         &     -0.0165\sym{***}&       0.601\sym{***}&       0.109\sym{***}&       0.118\sym{***}&      0.0400\sym{***}&    -0.00644\sym{*}  \\
                    &     (23.72)         &     (25.47)         &      (1.96)         &      (0.34)         &     (-7.10)         &     (29.00)         &     (41.28)         &     (22.53)         &      (9.83)         &     (-2.52)         \\
\midrule
Observations        &       28370         &       28370         &       28370         &       28370         &       28370         &       28370         &       28370         &       28370         &       28370         &       28370         \\
\bottomrule
\multicolumn{11}{l}{\footnotesize \textit{t} statistics in parentheses}\\
\multicolumn{11}{l}{\footnotesize \sym{*} \(p<0.05\), \sym{**} \(p<0.01\), \sym{***} \(p<0.001\)}\\
\end{tabular}
\end{adjustbox}
\end{table}

\end{document}
