# Supplementary material for: Breaking Down the Lockdown: The Causal Effects of Stay-At-Home Mandates on Uncertainty and Sentiments During the COVID-19 Pandemic
Source: arXiv:2212.01705 source file (2023-06-01)
Supplement: Supplementary file 6 [file intro_old_stuff.tex]

%Uncertainty and economic sentiment may damped the effectiveness of policies \autocite{Aastveit2017}. As effective as they are from a health perspective, lockdowns may generate uncertainty and fuel negative sentiments among individuals subject to this policy, leading to sizable economic, social and political externalities. Several studies have documented the negative externalities stemming from lockdown measures, such as higher inequality and economic burden \autocite{palomino2020wage}, worse mental health conditions \autocite{banks2020mental,elmer2020students}, increased doom-scrolling and social media addiction \autocite{anand2022doomsurfing}, lower public trust and political participation \autocite{Bonotti2021}, as well as political approval \autocite{Fazio2021political}. In this context, measuring the non-sanitary effect of lockdown policies is crucial for policy makers to thoroughly assess the benefits and costs of such measures. 
%To balance costs and benefits, policy makers must decide on the restrictions' optimal spatial location, duration and stringency based on health, economic, social and political considerations. As viruses evolve and new variants emerge, it is of the upmost importance for policy makers to plan for strategies promoting a long-term sustainable balance between effective, possibly targeted, public health interventions and adverse social, economic and political externalities. In this context, measuring the effect of a lockdown policy on the public's uncertainty and sentiments provides vital information about the effectiveness the policy from a non-sanitary perspective.

%In this paper, we estimate the effects of a lockdown policy on economic, social and political uncertainty and sentiments. Uncertainty is highly relevant due to its negative economic implications on financial volatility, investment, employment, output, bank credit, and capital flows \autocite{Baker2016, pastor2013political, bruno2015cross, Choi2023}. Moreover, uncertainty can dampen the effectiveness of policies \autocite{Aastveit2017}. In particular, uncertainty over the lockdown restrictions and the subsequent circulation of false information has been shown to account for a large portion of the negative turnout of economic activities during the pandemic \autocite{RePEc:sgh:kaewps:2021060}. Low readability of the official information and contradicting statements produced psychological distress and confusion among the public \autocite{healthcare8030249}, which indicates that the policy may not have been well understood and its effectiveness dampened. Mishra and Dexter \autocite{mishra2020comparison} analysed agency sites and 15 official government sites of countries official information about COVID-19 early into the first wave of the COVID-19 pandemic (April 2020), finding that official information exceeded the recommended reading level in all counties. Interestingly, Italian official information exhibited the most complex syntax (as measured via the mean length of clause), ranked among the least readable (with respect to five different readability indicators) and made extensive usage technical terminology. The authors argue that this might have had a great influence in exacerbating the disparate effects and externalities of the pandemic. Furthermore, the COVID-19 pandemic period has led to high policy uncertainty in states under stricter lockdown measures \autocite{NBERw29714}. However, the causal effect of lockdown policies on people's perceived uncertainty and sentiment has not been estimated yet. 

%On the other side, identifying the public discontent is crucial to monitor the public support to the lockdown policies and the public entities enacting these policies. As highlighted by the reactions to Chinese targeted lockdown policies, the imposition of tight restrictions on movements and activities intensified negative sentiments among economic agents \autocite{doi:10.1080/00036846.2022.2061903} and the countries hit the most by the economic downfall were those that experienced the hardest shift in sentiments \autocite{VANDERWIELEN2021105970}, supporting the idea that the policy did not boost the public's confidence towards the government's ruling.  
%Furthermore, monitoring public debate via social media represents a fundamental tool for a successful management of public emergencies. By collecting and analysing information coming from a huge stream of online exchanges, governments can learn how a policy is perceived, where the public's concern lies and which topics are associated to higher distress, to efficiently target and act upon public needs by adjusting interventions to changes in public sentiment \autocite{10.1057/s41599-022-01181-w, https://doi.org/10.48550/arxiv.2005.11458}.



% EMPIRICAL STRATEGY: vrs 15-05-2023 


\section{Empirical Strategy} 


Our aim is to measure the effect of the lockdown on uncertainty and negative sentiments in the public. To this end, we exploit the exogenous shock of the unexpected lockdown measures enacted in the red zone on February 23rd, 2020. 

Let $i$ be a tweet - our unit of observation, $T$ be the time period at which we observe units, $T_{i} = t$ for t periods, with $t=0,1,2$---i.e., before ($t=0$) and after ($t=1$) the implementation of the lockdown of February 23rd and following the nation-wide measures of March 9th ($t=2$).

We adopt a Difference-in-Differences (DiD) approach \autocite{RePEc:cup:cbooks:9780521848053} and estimate the following equation on repeated cross-sections of tweets:
\begin{equation}
Y_{i,t} = \alpha + \gamma D_{i} + \sum_{t \in \{1,2\}}\lambda_{t}\bbone[T_{i} = t] + \sum_{t \in \{1,2\}}\delta_{t}(\bbone[T_{i} = t] \times D_{i}) + \epsilon_{i,t} 
\end{equation}
where the time period dummies $\lambda_{t}$ indicate the pre-post-post lockdown periods and $\gamma$ represents the treatment group-specific effect, which accounts for average permanent differences between units treated in period 1 and non-treated in period 1. Our coefficient of interest is $\delta_{1}$, whose OLS estimated coefficient is given by:
\begin{equation}
    \hat{\delta_{1}}  =\frac{1}{N_{T}}\sum_{i: D_{i} = 1}(Y_{i,1} - Y_{i,0}) - \frac{1}{N_{C}}\sum_{i: D_{i} = 0}({Y_{i,1} - Y_{i,0}})
\end{equation}
where $N_{T}$ is the total number of treated units and $N_{C}$ the number of control units
The OLS coefficient $\hat{\delta_{1}}$ becomes a consistent estimator of the average treatment effect ATT(1) under assumptions (1), (2) and (3).

%In our DiD setting, the average treatment effect on the treated in period 1---i.e. ATT(1)---is the causal estimand of interest, defined as
%\begin{equation}
%    ATT(1)  = \EX[Y_{i,1}(1) - Y_{i,0}(0) | D_{i} = 1] 
%\end{equation} 

Because it is possible to observe only $Y_{i,1}(1)$, the identification strategy of the DiD approach imputes the unobserved potential outcomes for the treated units with the \emph{observed} post-treatment outcomes for untreated units that are suitable \emph{counterfactuals} of what would have happened to the treatment units if they were not treated. 


As the control units eventually become treated once the measures are extended nationwide, our setting features a \emph{staggered} treatment timing, where units receive treatment at different time periods. In Model (3), the coefficient $\delta_{t}$ is equivalent to a \cite{CALLAWAY2021200} estimator returning the average treatment effect at time t for units treated for the first time at time $t$. 

Following \cite{CALLAWAY2021200}, let $G$ be a time period indicator when a unit starts treatment. Define $G_{i,g}$ as a binary variable indicating whether unit $i$ received the treatment for the first time in period $g$, and $D_{i,t}=\bbone[T = t] \times D_{i}$, indicating whether unit $i$ is treated at time $t$. When the identifying assumptions of (i) no treatment anticipation and (ii) parallel trends based on \emph{not-yet treated groups} hold unconditionally on covariates, the causal estimand of the average treatment effect is given by

\begin{equation}
    ATT(g,t) =  \EX[Y_{i,t} - Y_{i,g-1} | G_{i,g} = 1] - \EX[Y_{i,t} - Y_{i,g-1} | D_{i,t} = 0]
\end{equation}
for $g \leq t < \hat{g} = max_{1,...,n}\{G_{i}=g\}$---i.e. for $t$ between the last period in which a new group enters treatment and the time of first entering treatment\footnote{We refer to \cite{CALLAWAY2021200} for details on the generalization of Assumptions 1 and 2 in a staggered DiD setting.}. This estimator measures the changes in outcomes between the current period and the first period preceding the treatment ($g-1$), comparing units firstly treated at time $g$ and those yet-to-be treated at time $t$. This means that $ATT(g,t)$ cannot be identified for time periods after the very last treatment group starts the treatment, nor we can identify the treatment effect for this last treatment group, as we lose any counterfactual quantities. 

The estimand in (5) generalizes the standard two-group, two-periods DiD estimator, where the not-yet-treated group is taken as a suitable counterfactual group. In our setting, $t \in \{0,1,2\}$, $\hat{g} = 2$ and the appropriate time reference is $t = 0$. Then it follows that
\begin{equation}
    ATT(1,1) =  \EX[Y_{i,1} - Y_{i,0} | G_{i,g} = 1] - \EX[Y_{i,1} - Y_{i,0} | D_{i,1} = 0] = ATT(1)
\end{equation} 
The equality holds only for $t < 2$, that is, for $t = 1$, as we are able to identify the average treatment effect for $t=1$ for treatment units starting treatment in period $t=1$. The coefficient $\delta_{2}$ cannot be identified as the average treatment effect on the second cohort of treated units, as there are no longer any untreated units available for constructing counterfactuals. Instead, the OLS estimate of $\delta_{2}$ can inform us of the influence of initial exposure to treatment, if the effect for those longer exposed to treatment is the same for those just starting treatment. We cannot talk about the \emph{dynamic heterogeneity} of treatment when interpreting $\delta_{2}$, as we are making a forbidden comparison between two treated groups, we can just infer on the difference in outcome between those in the first and the second treatment cohort in the last treatment period.
%Considering that we have only two treatment periods, $t=1,2$, the observed potential outcome at time t is given by  $Y_{i,t} = Y_{i,1}(0) + G_{i,1}(Y_{i,t}(1) - Y_{i,t}(0)+ G_{i,2}(Y_{i,t}(2) - Y_{i,t}(0))$ -- i.e. we can only observe the outcome for treated units when the unit enters treatment at time $t$ and the outcomes for the untreated at time $t$. 



\subsection{Assumptions}
 
Let $i$ be a tweet - our unit of observation, $T$ be the time period at which we observe units, $T_{i} = t$ for t periods, with $t=0,1,2$---i.e., before ($t=0$) and after ($t=1$) the implementation of the lockdown of February 23rd and following the nation-wide measures of March 9th ($t=2$). Units are assigned to the targeted lockdown in period $t=1$, while at $t=2$ all units become treated. Define $D_{i}$ as the \emph{treatment status} indicator, equal to 1 if unit i is subject to the lockdown of February 23rd---i.e. the \emph{treatment}---zero otherwise. Let $Y_{i,t}$ be the binary outcome variable observed for unit $i$ in period $t \in \{0,1,2\}$. $Y_{i,t}(0)$ represents the potential outcome of unit $i$ in period 1 if they remain untreated at time $t$, $Y_{i,1}(1)$ the potential outcome at time $t$ if they were treated at time $t$. For each unit, we can only observe one of the potential outcome at each time period. %Therefore, the observed outcome is given by $Y_{i,t}=(1-D_{i})Y_{i,t}(0)+D_{i}Y_{i,t}(1)$ for $t=0,1$, as, under our setting, at time $t=2$ \emph{all} units are treated and therefore $Y_{i,2}=Y_{i,2}(1)$. 

The average treatment effect on the treated in period 1---i.e. ATT(1)---is the causal estimand of interest, defined as
\begin{equation}
    ATT(1)  = \EX[Y_{i,1}(1) - Y_{i,0}(0) | D_{i} = 1] 
\end{equation} 

We can estimate the ATT(1) by making the following assumptions:

\begin{assumption}
Parallel Trends: 
\begin{equation*}
    \EX[Y_{i,1}(0) - Y_{i,0}(0) | D_{i} = 1] - \EX[Y_{i,1}(0) - Y_{i,0}(0) | D_{i} = 0].
\end{equation*}
\end{assumption}
In other words, in absence of the treatment, the outcome in the treated group would have followed the same trend as the control group. This assumption requires that units belonging to treated and control two groups should not exhibit there no inherent, systematic differences, such that we can exclude any \emph{selection bias} in the estimation of the treatment. 

\begin{assumption}
No anticipation of the treatment: 
\begin{equation*}
    Y_{i,0}(1) = Y_{i,0}(0) 
\end{equation*}
for all treated units i $D_{i} = 1$.
\end{assumption}
This assumption implies that before the treatment, the treatment does not impact the outcomes of the treated units -- i.e. units cannot modify their outcomes in order to be selected into treatment.

\begin{assumption}
\emph{Stable Unit Treatment Values Assumption} (SUTVA)
\begin{equation*}
ATT(1) =  \delta_{1} + \delta^{spill}_{1}(1) - \delta^{spill}_{1}(0) = \delta_{1}
\end{equation*}
\end{assumption}
where $\delta^{spill}_{1}(1)$ is the average spillover effect on treated units and $\delta^{spill}_{1}(0)$ the average spillover non-treated units in period 1, which are set to zero under SUTVA. The treatment assignment or the potential outcome of a unit cannot affect the potential outcome of another unit.

Under these assumptions, it follows that:
\begin{equation}
    ATT(1)  = \EX[Y_{i,1} - Y_{i,0} | D_{i} = 1] - \EX[Y_{i,1} - Y_{i,0} | D_{i} = 0]
\end{equation}
provided that units are drawn at random from a larger population.
%and unit's treatment assignment has no \emph{spillovers} effect on nearby units\footnote{In Section D of the Appendix, we discuss into detail the parallel trend assumption and conditions for violation of the SUTVA.} \autocite{roth2023whats}.



% Abadie: as there is clustering in the treatment assignment, as unit's treatment status is perfectly correlated within clusters. Therefore one should cluster at the level at which units are assigned independently to treatment.
%In our setting, units within the same cluster have all the same probability of being treated, which indicates that the treatment assignment is \emph{perfectly} correlated within clusters. 

%the probability of treatment assignment within same cluster is 1 for all units = treatment assignment is correlated within clusters. 
